# Supplementary material for: VGGT-Motion: Motion-Aware Calibration-Free Monocular SLAM for Long-Range Consistency
Source: arXiv:2602.05508 source file (2026-02-05)
Supplement: Supplementary file 1 [file mono.pdf]

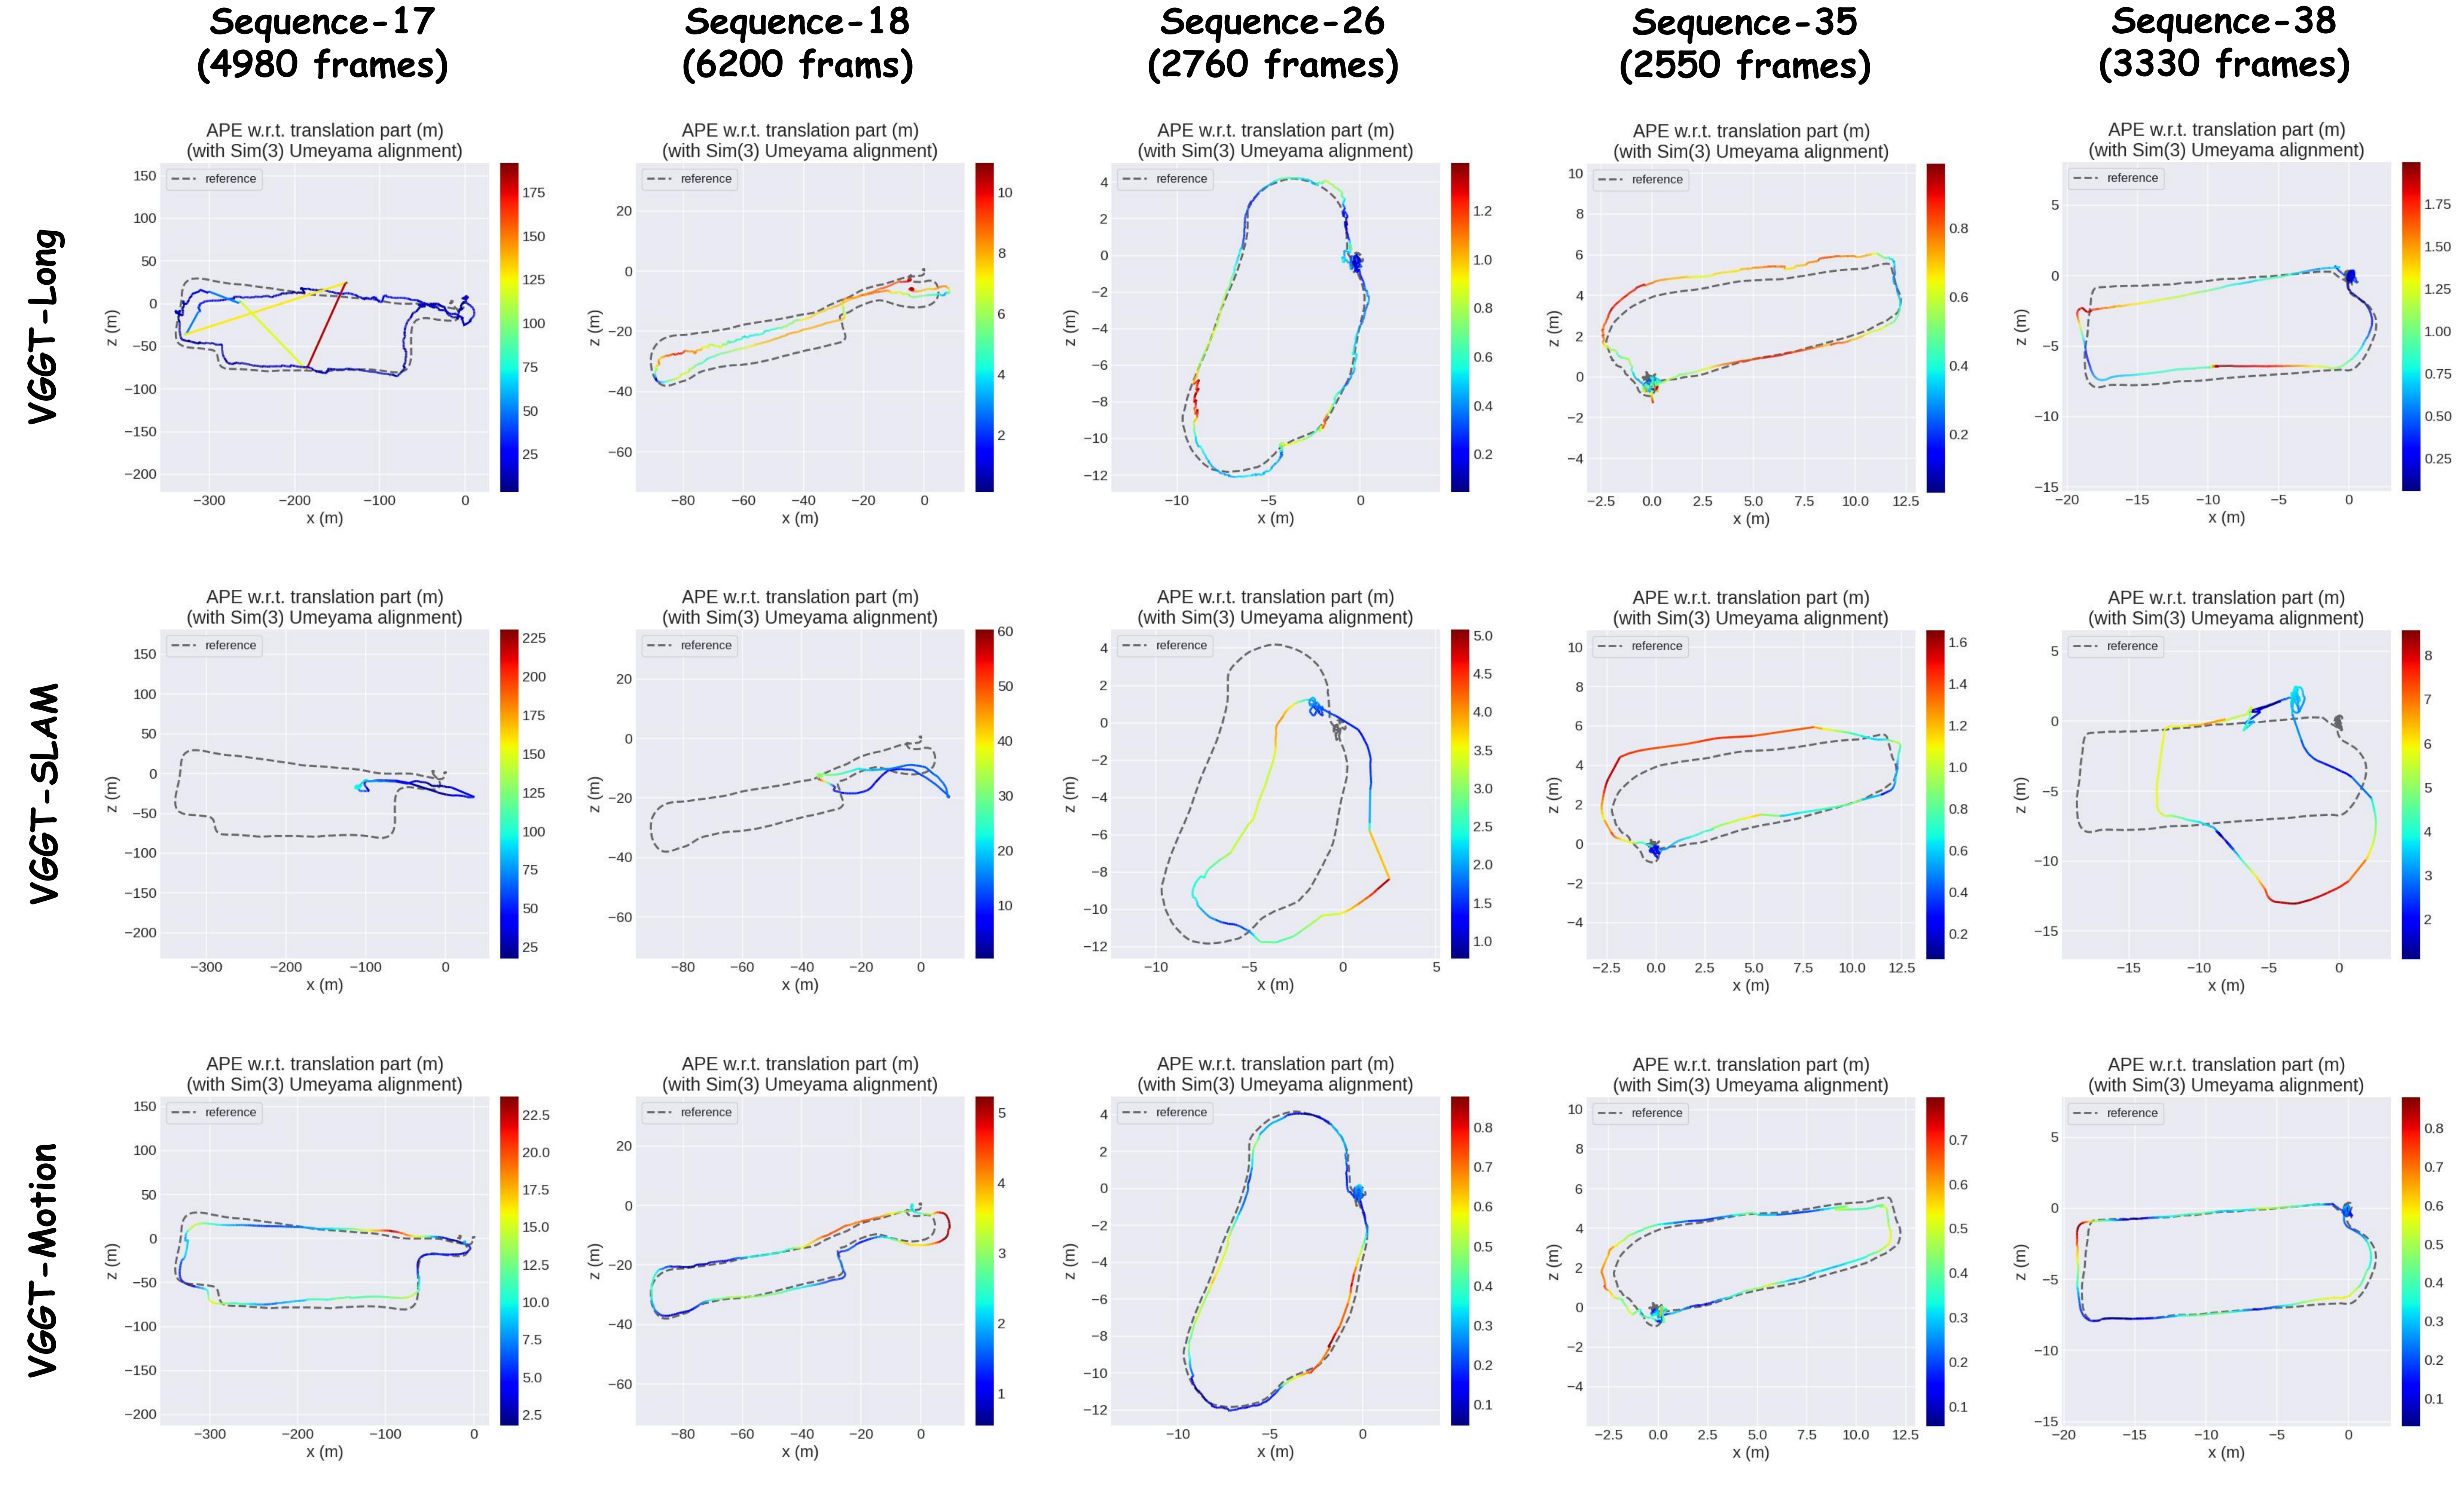

Sequence-17
(4980 frames)
Sequence-18
(6200 frams)
Sequence-26
(2760 frames)
Sequence-35
(2550 frames)
Sequence-38
(3330 frames)
VGGT-Long
VGGT-SLAM
VGGT-Motion
APE w.r.t. translation part (m)
(with Sim(3) Umeyama alignment)
reference
x (m)
z (m)

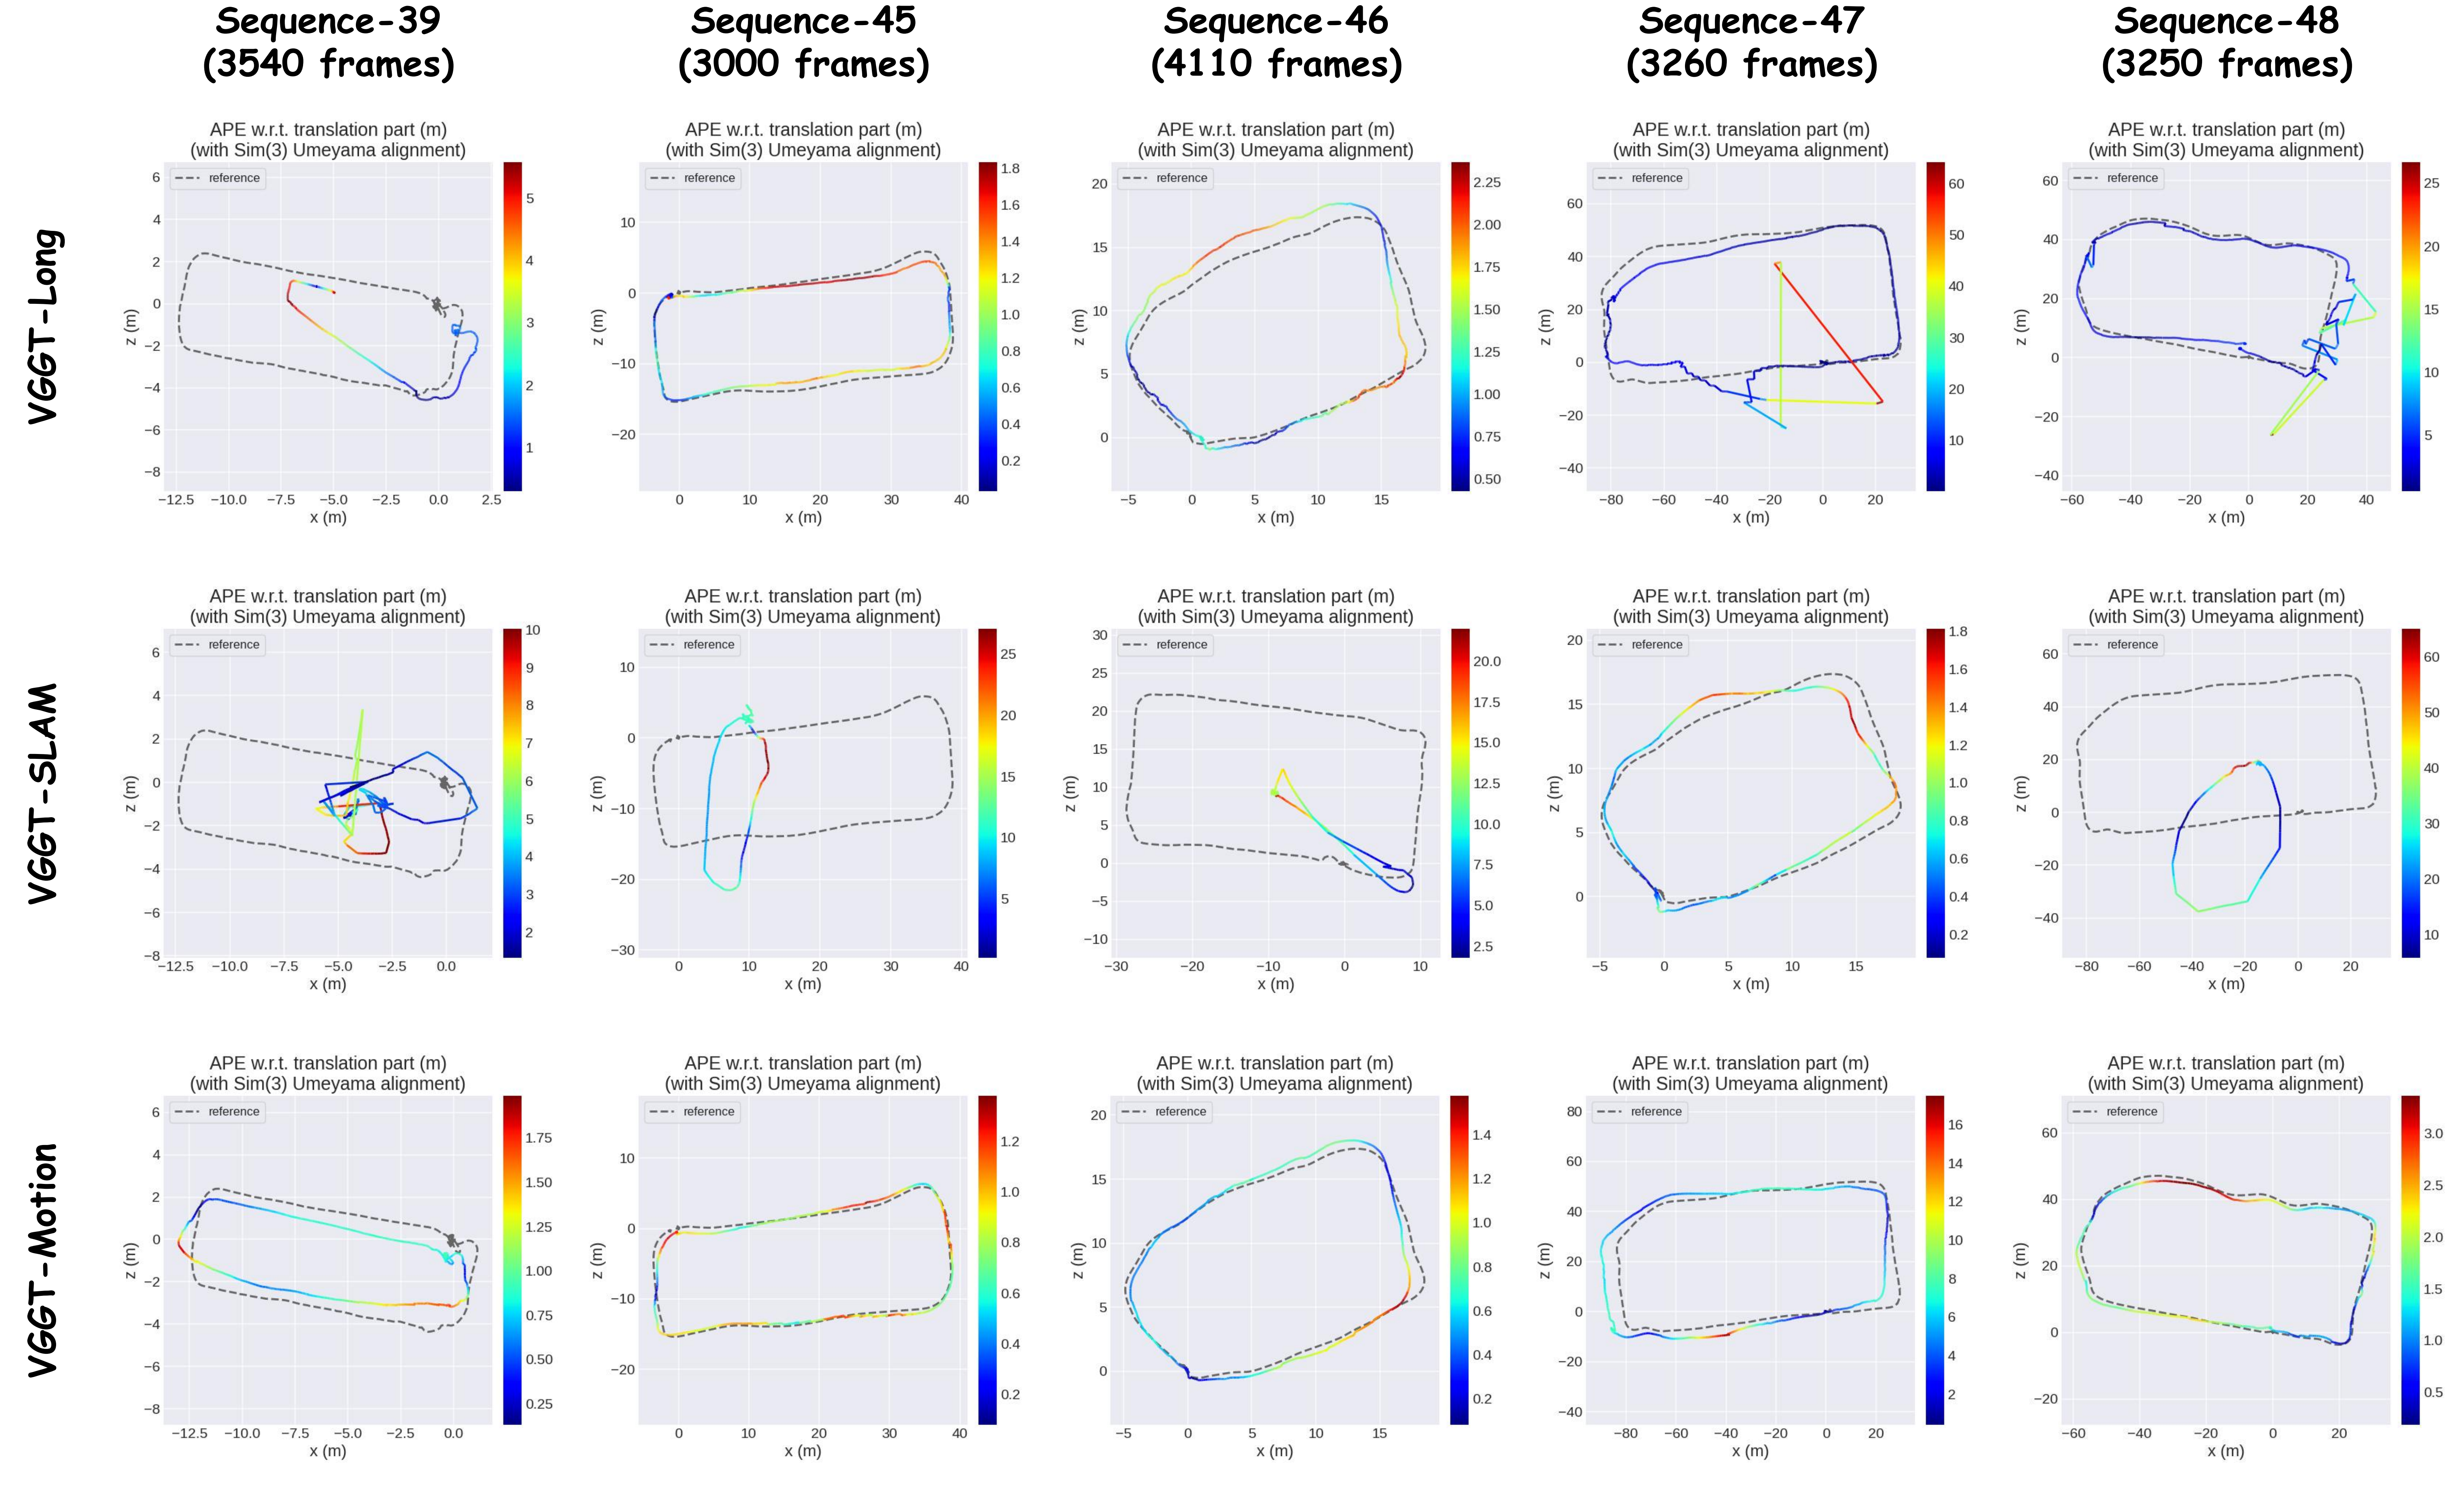
Sequence-39 (3540 frames)
Sequence-45 (3000 frames)
Sequence-46 (4110 frames)
Sequence-47 (3260 frames)
Sequence-48 (3250 frames)
VGGT-Long
VGGT-SLAM
VGGT-Motion
APE w.r.t. translation part (m) (with Sim(3) Umeyama alignment)
reference
x (m)
z (m)
