# Supplementary material for: VGGT-Motion: Motion-Aware Calibration-Free Monocular SLAM for Long-Range Consistency
Source: arXiv:2602.05508 source file (2026-02-05)

# Segment-163453191 (159.963 m)

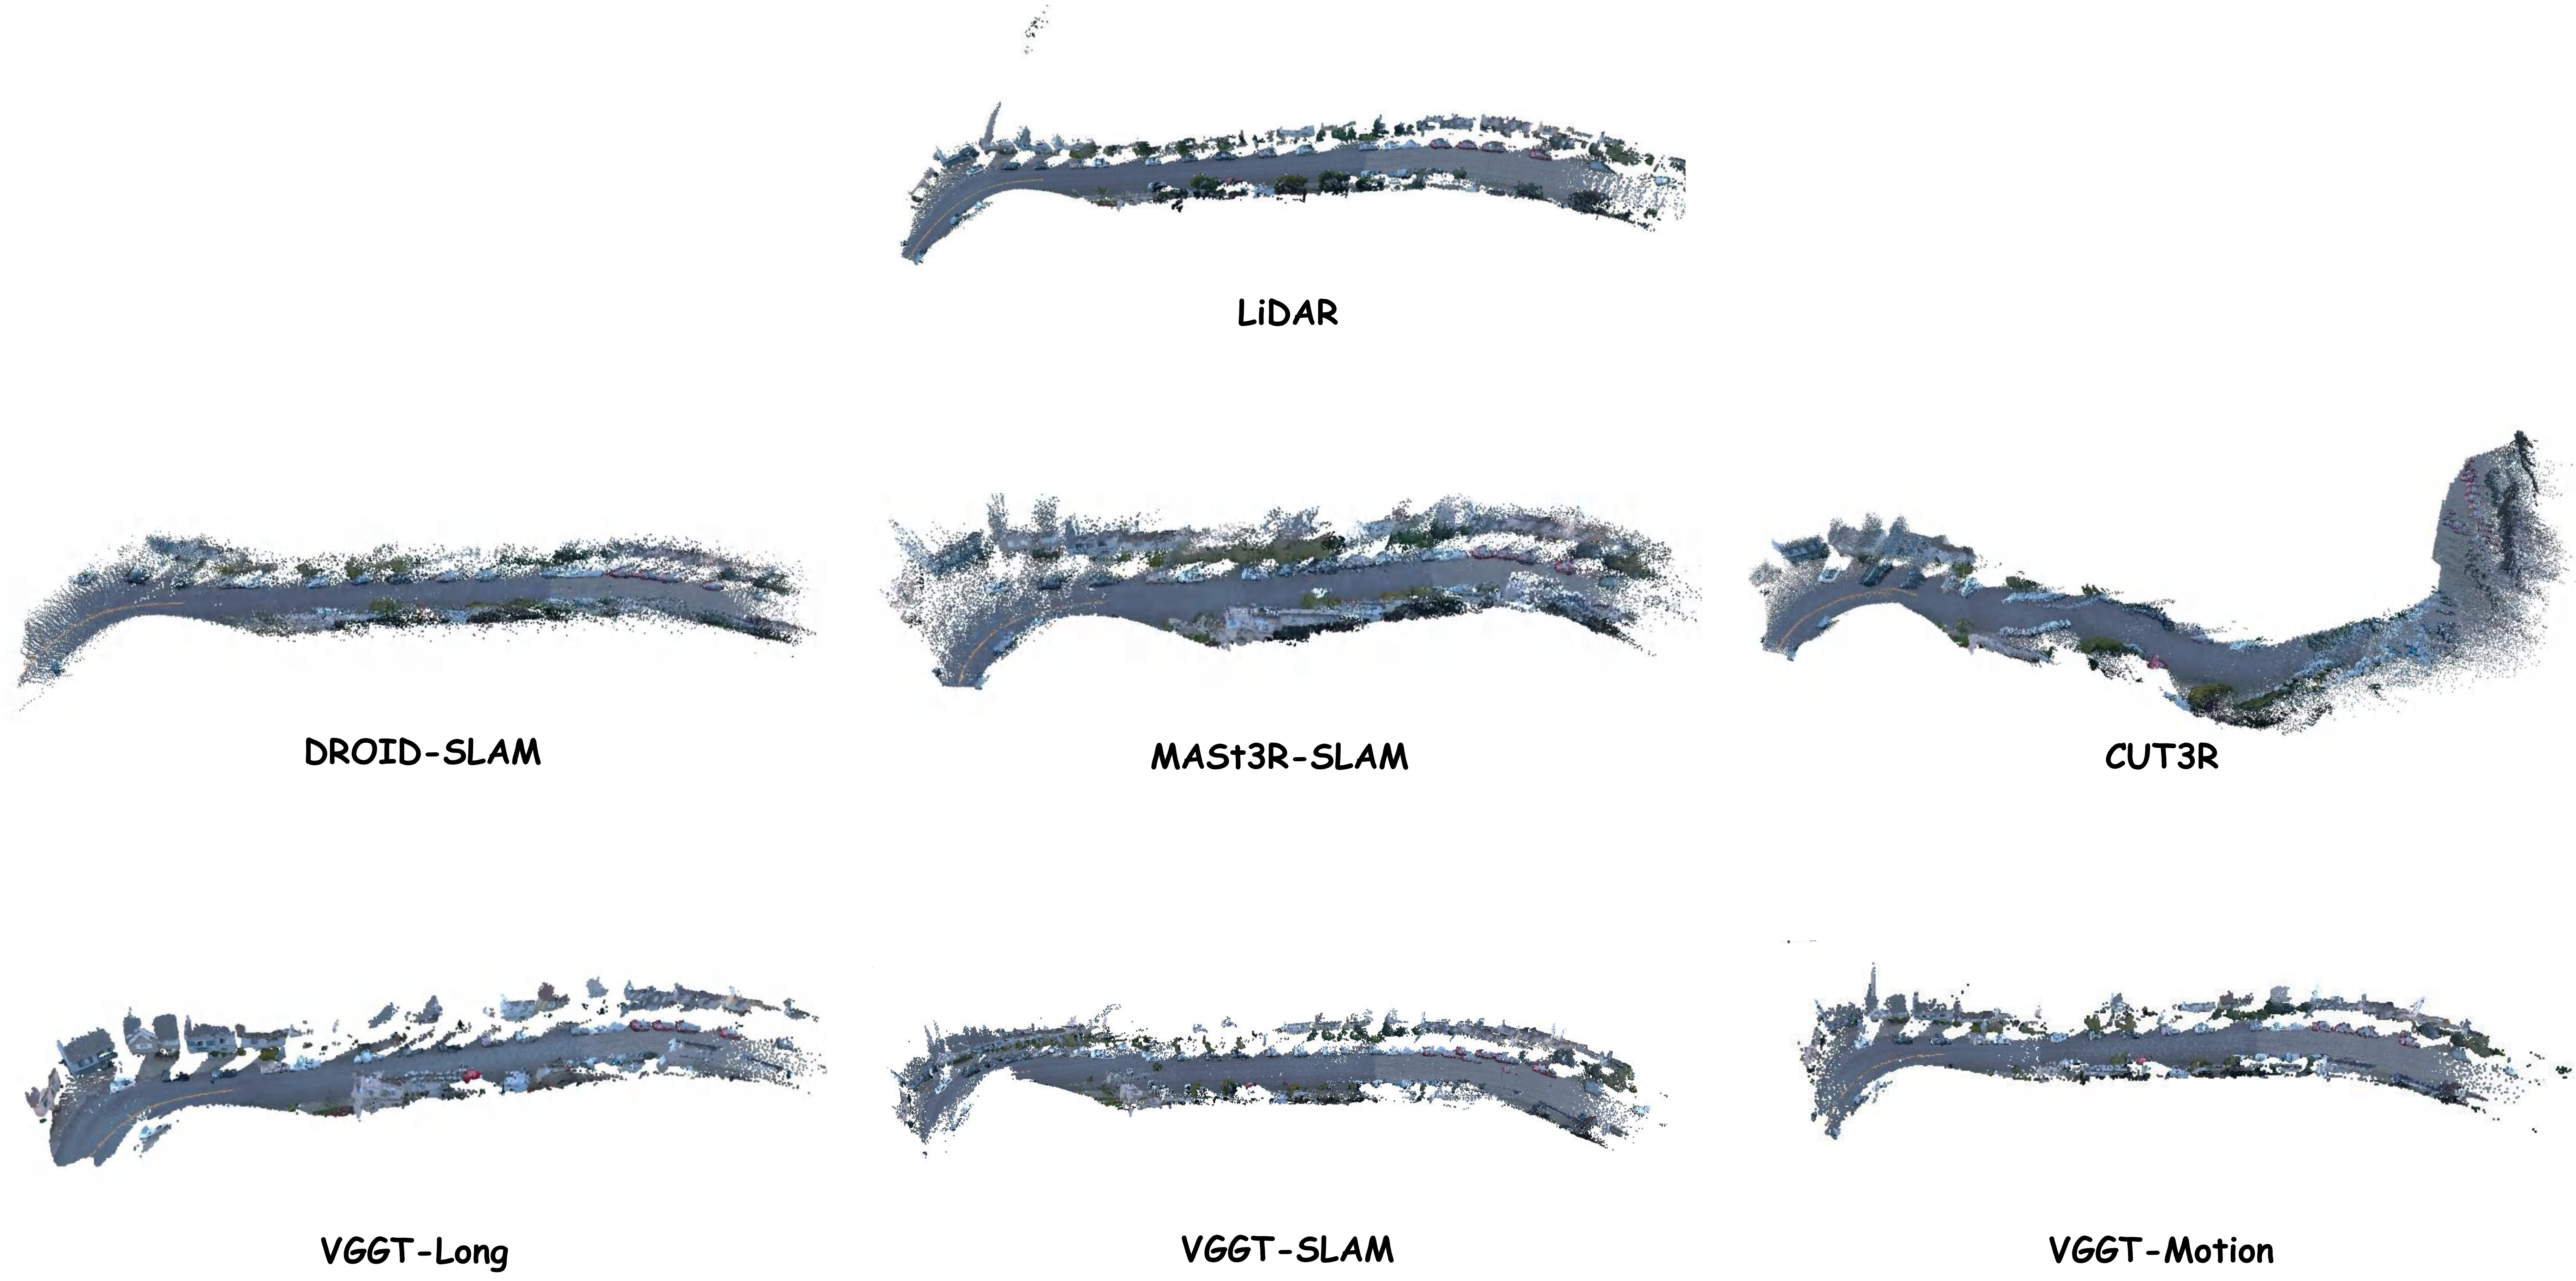

# Segment-183829460 (42.301 m)

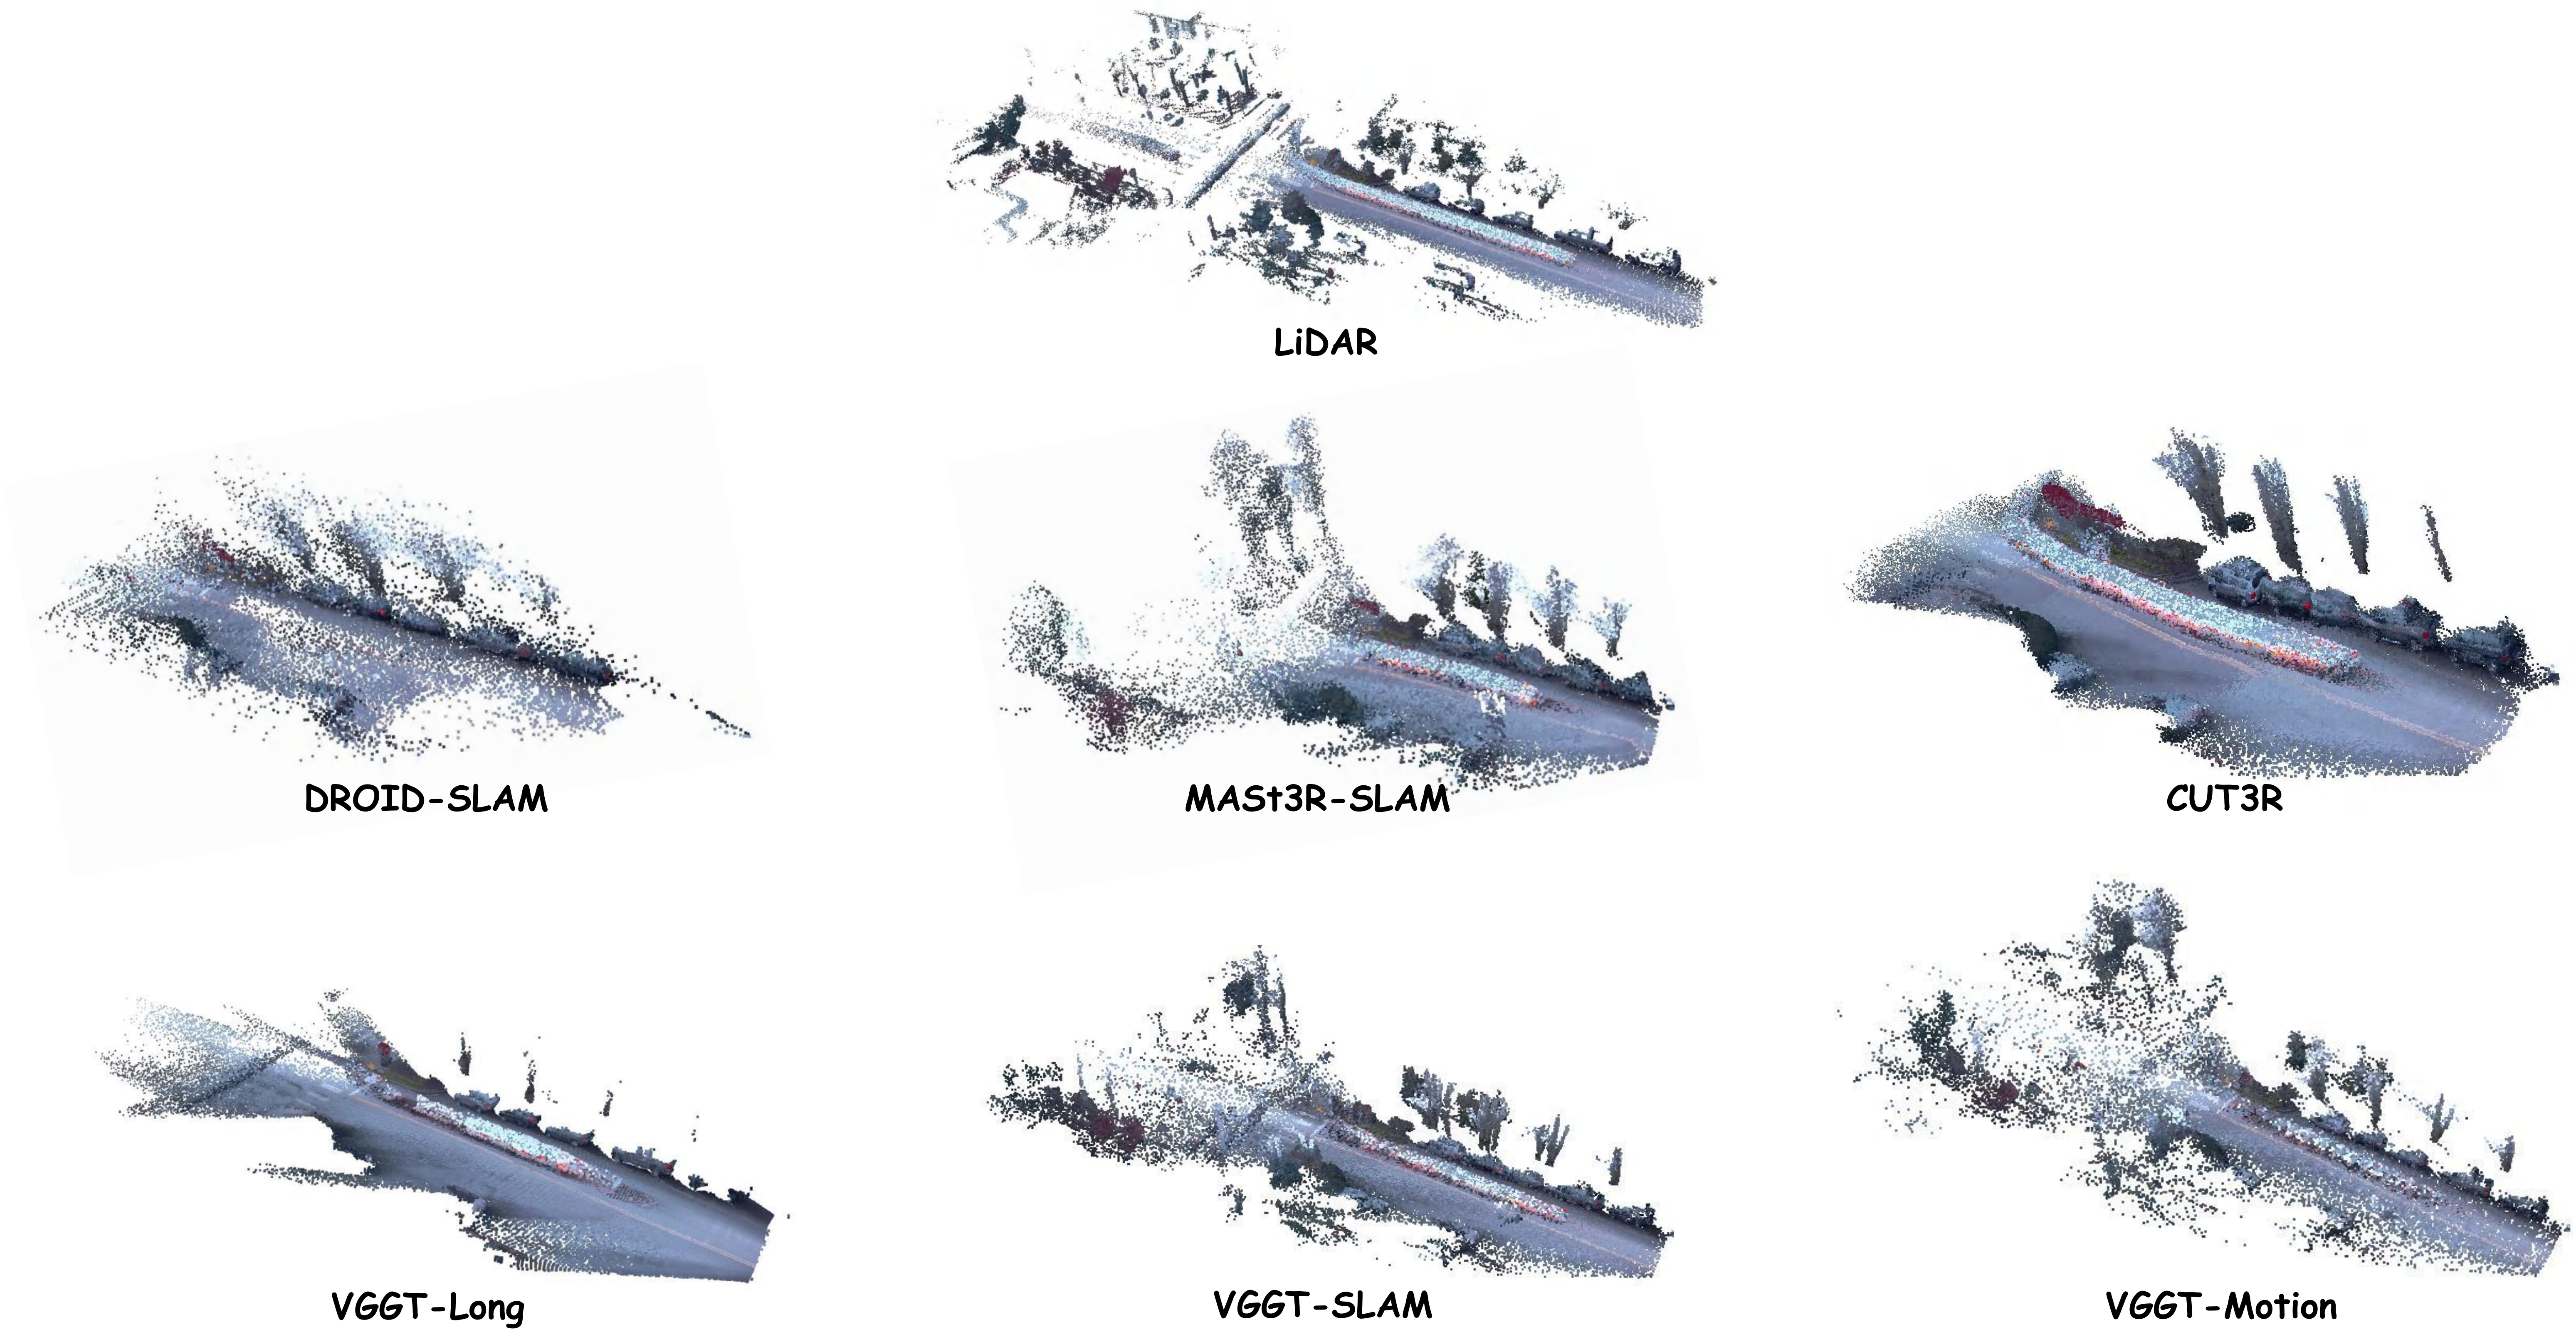

Segment-315615587 (165.149 m)

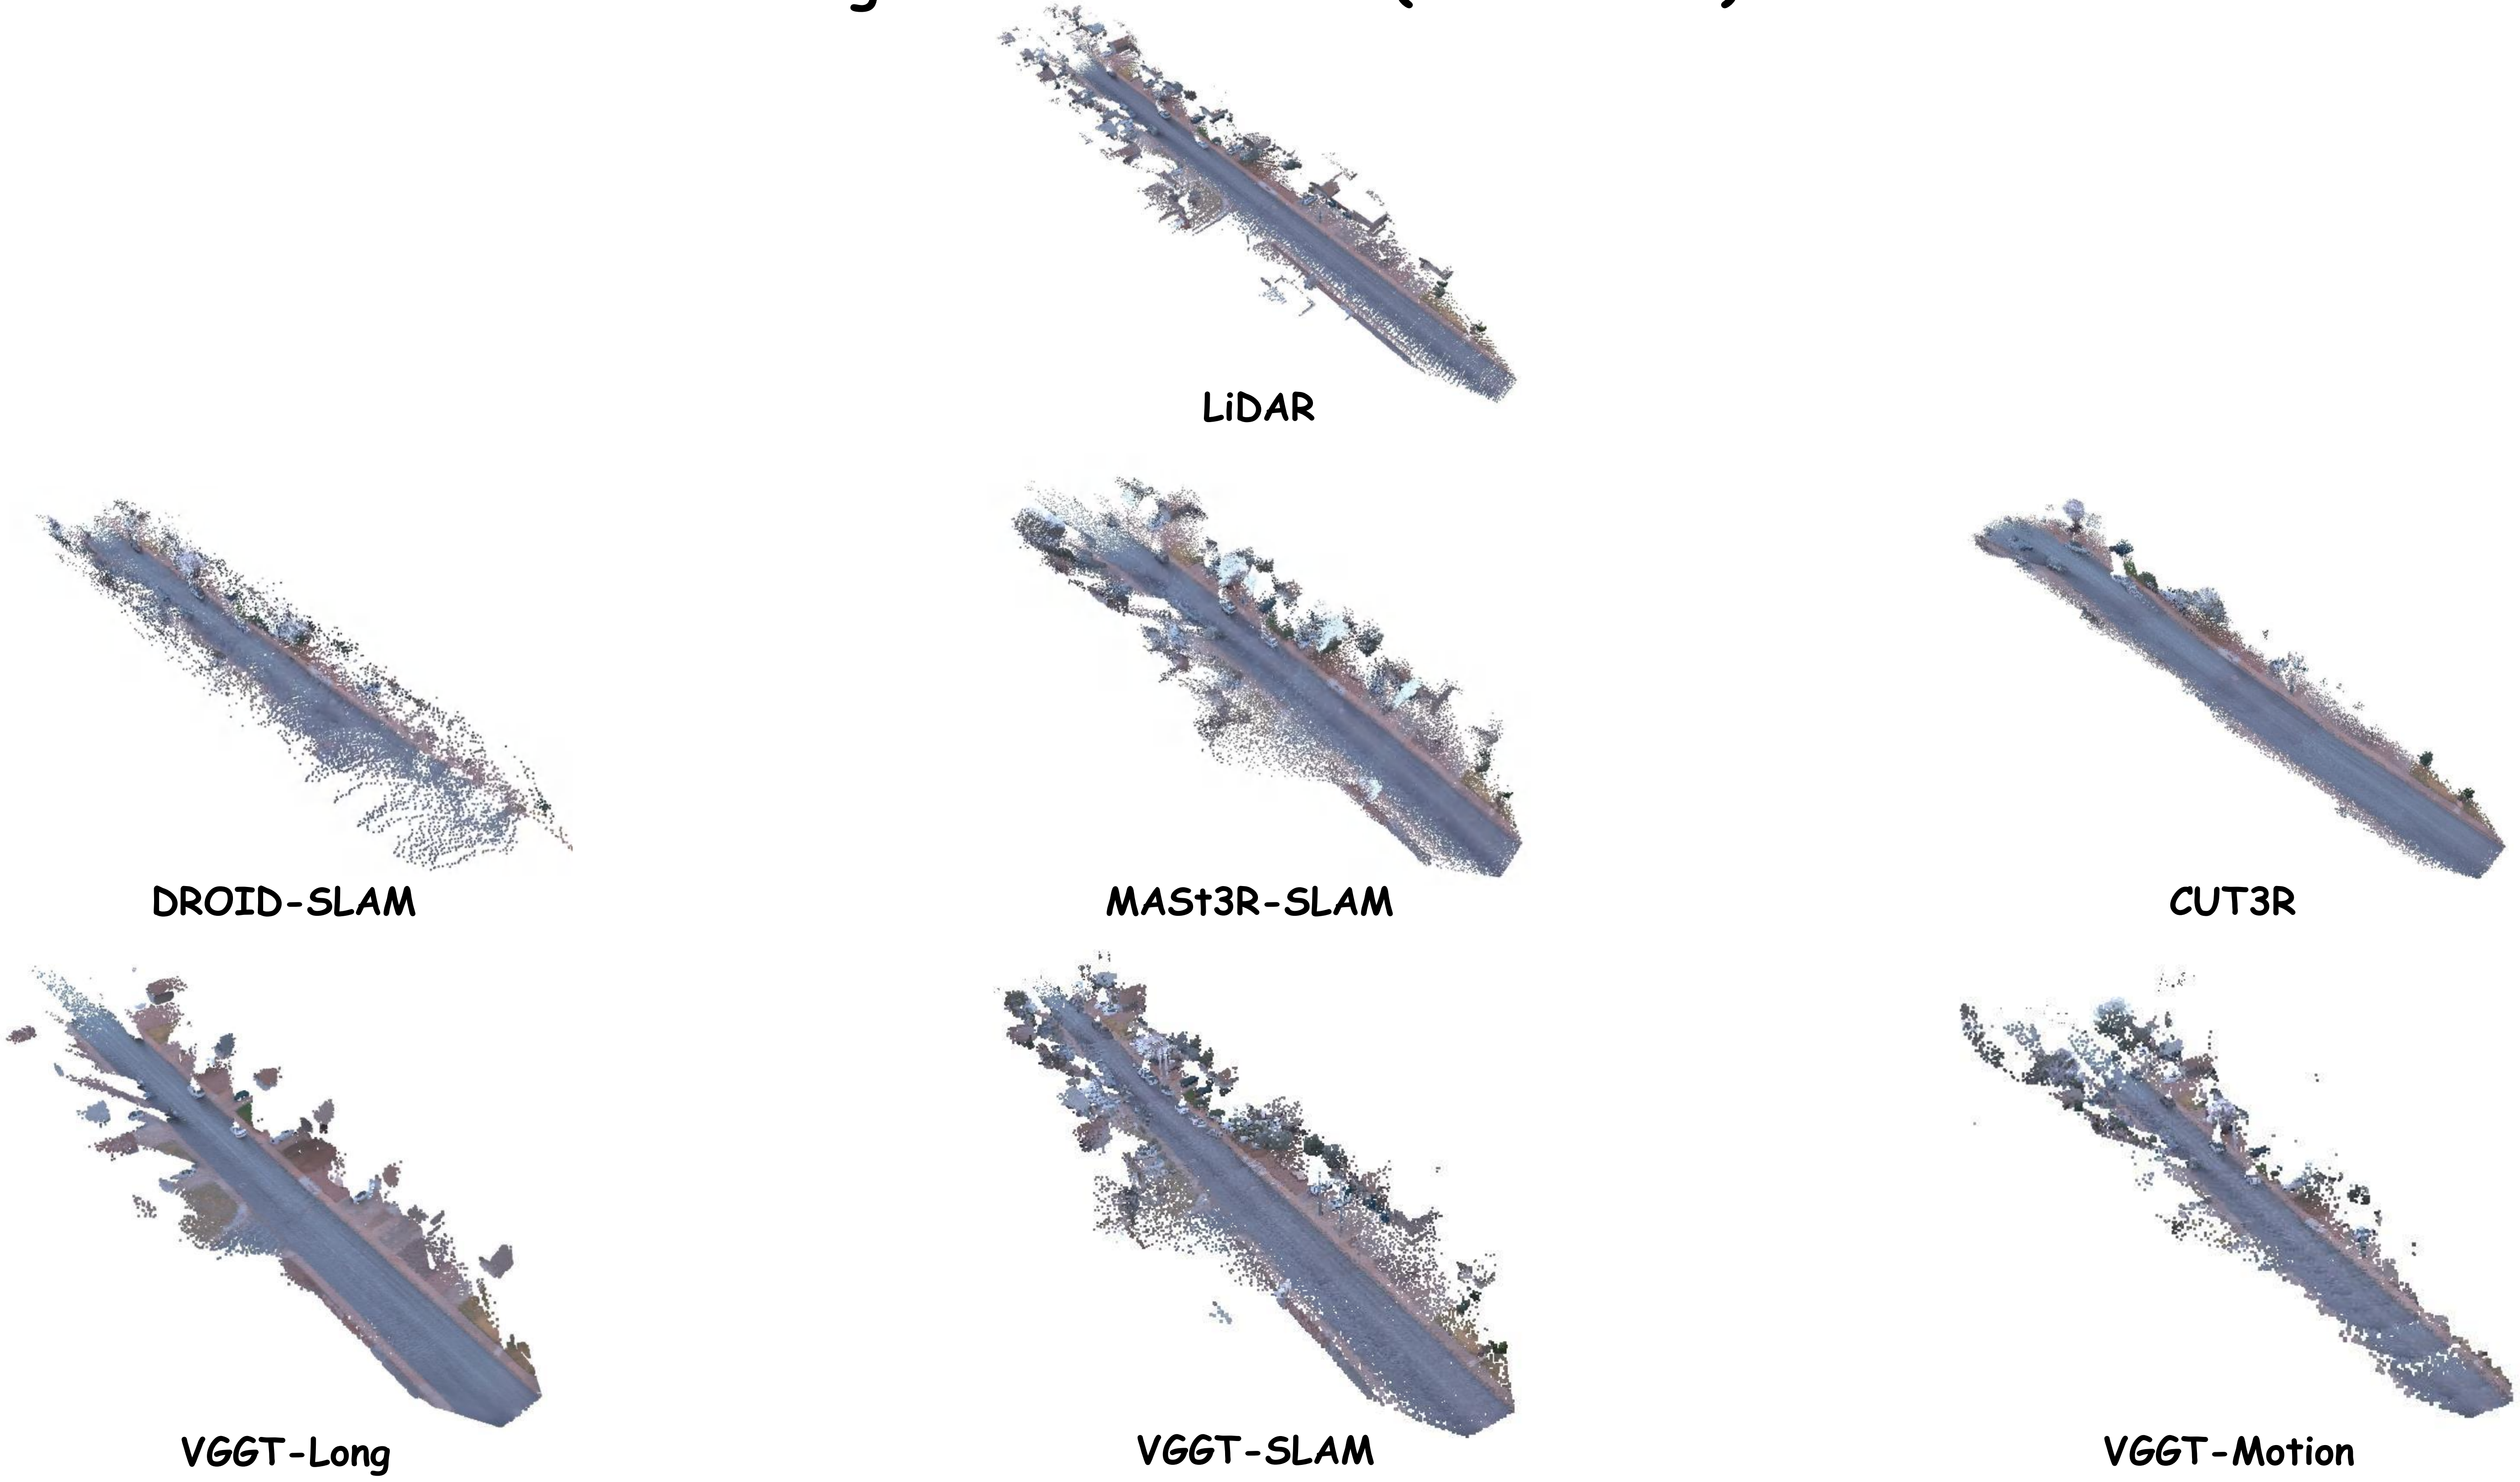

# Segment-346181117 (351.213 m)

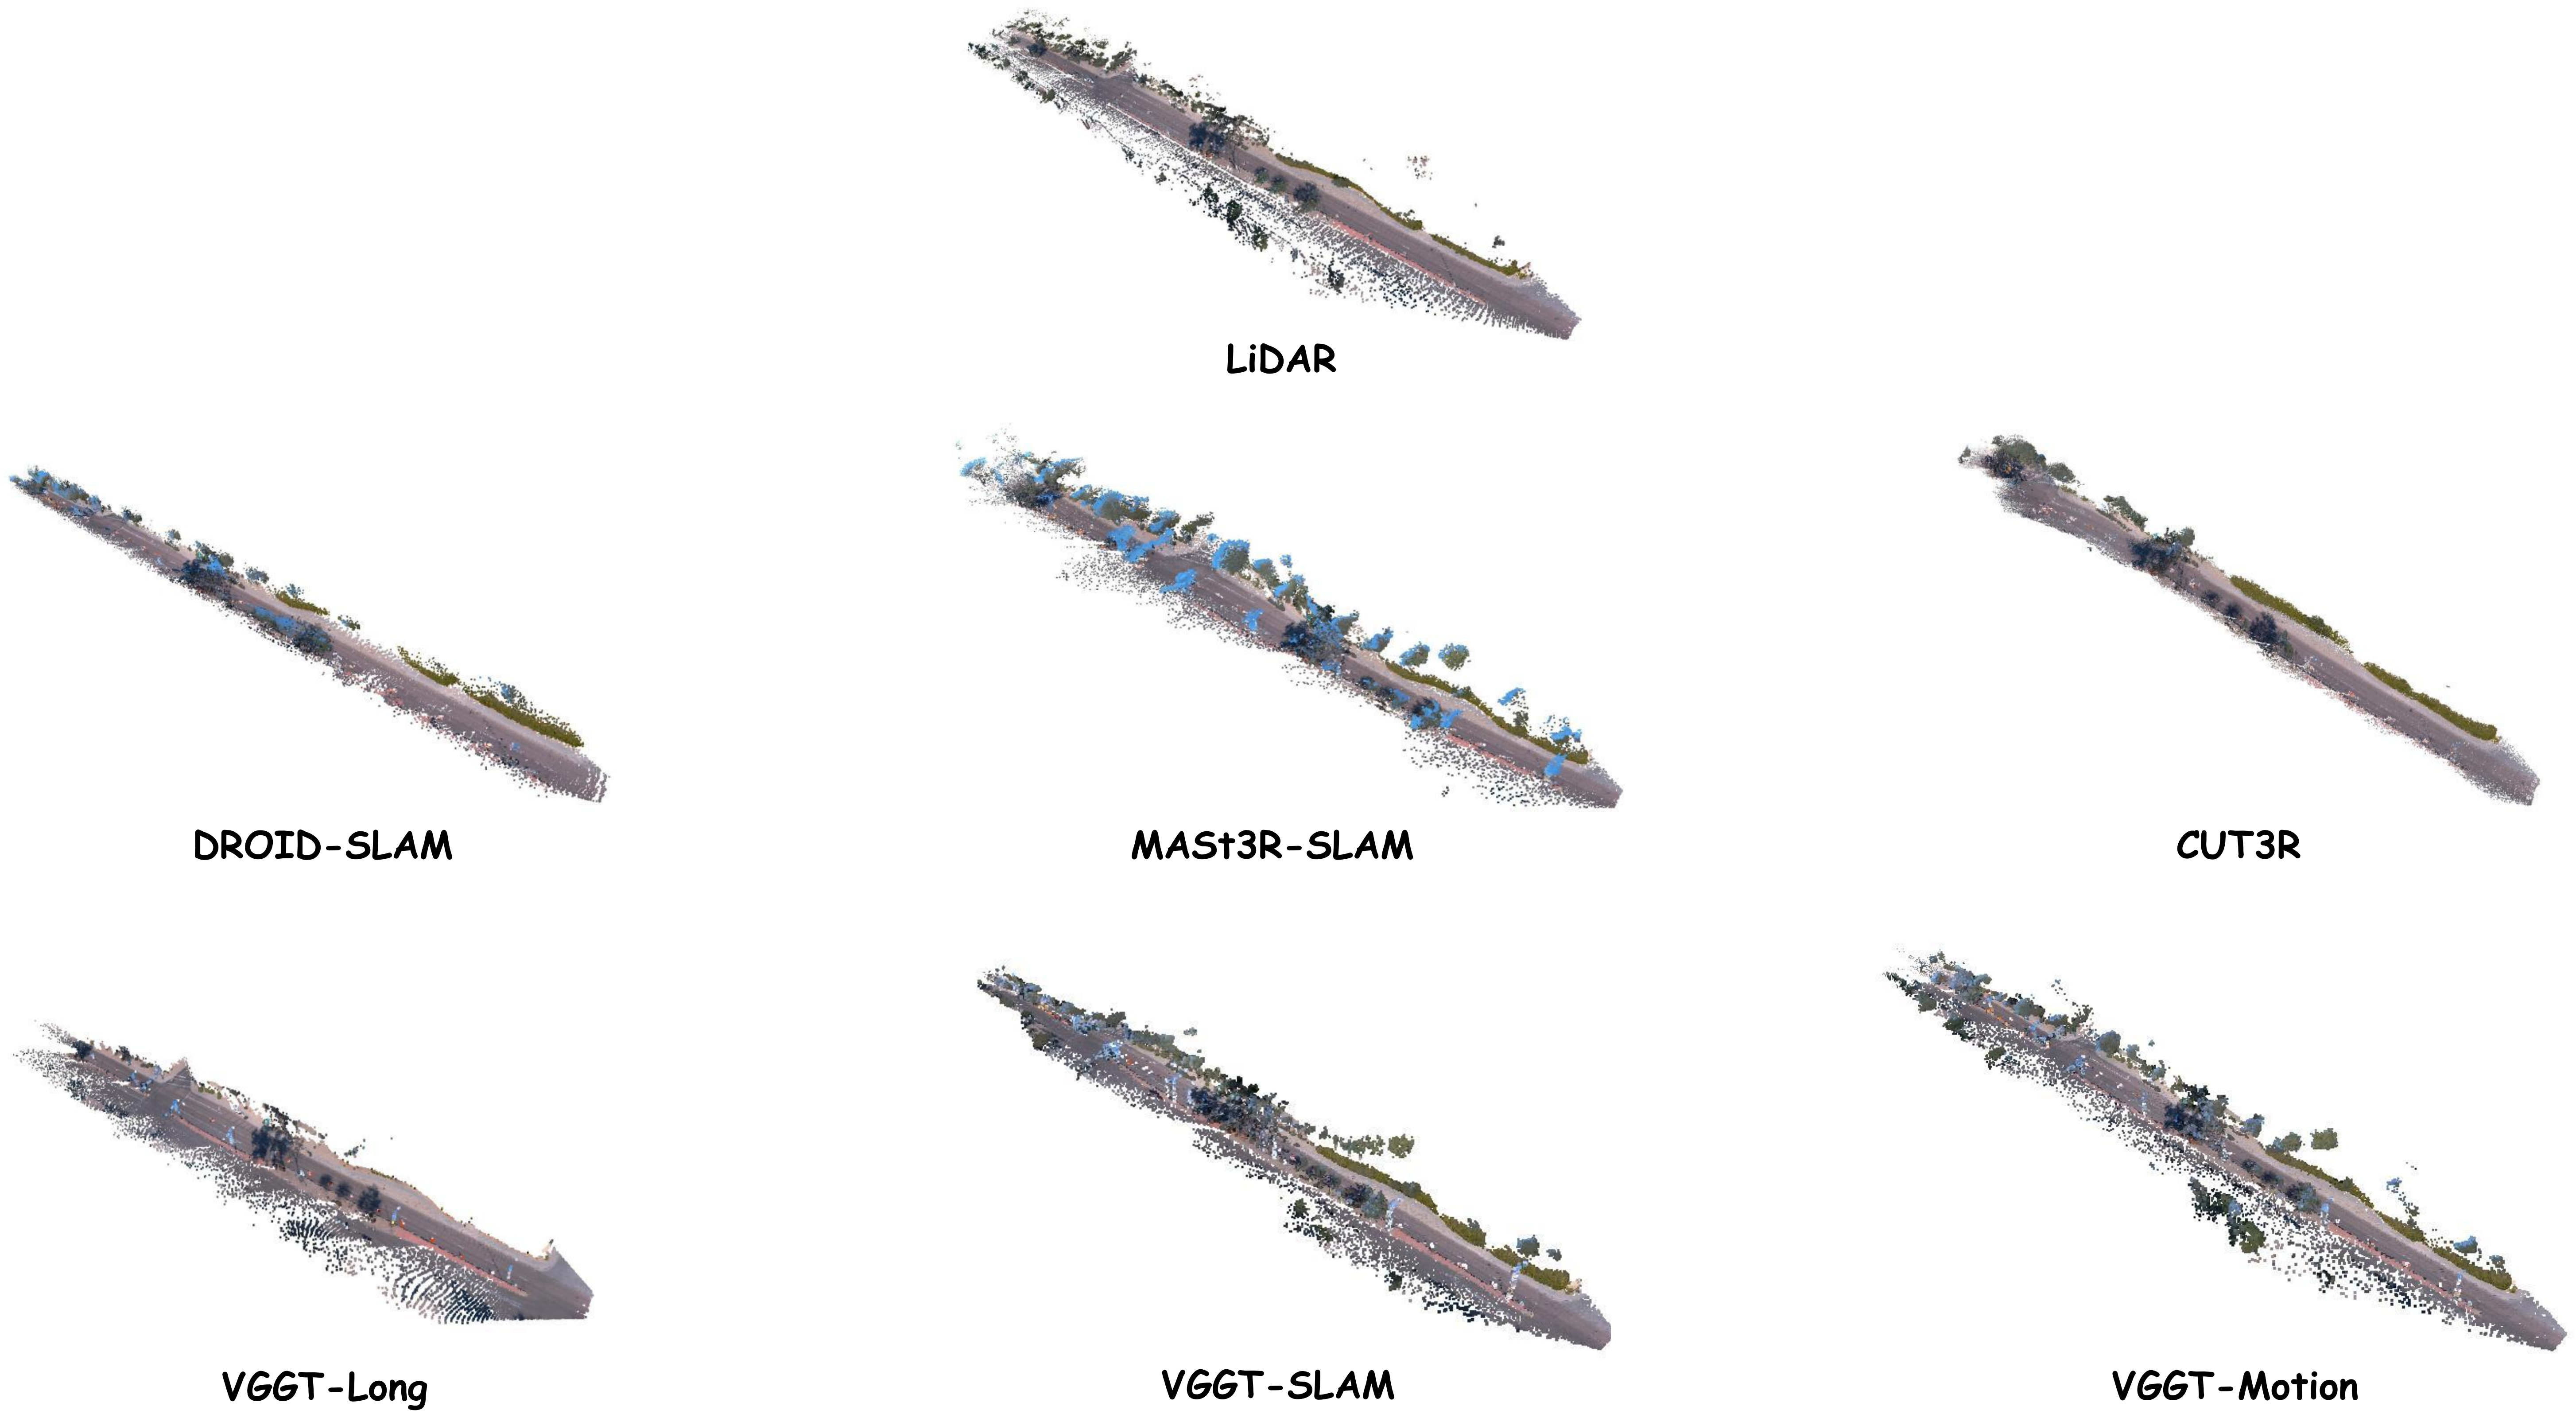

# Segment-371159869 (272.661 m)

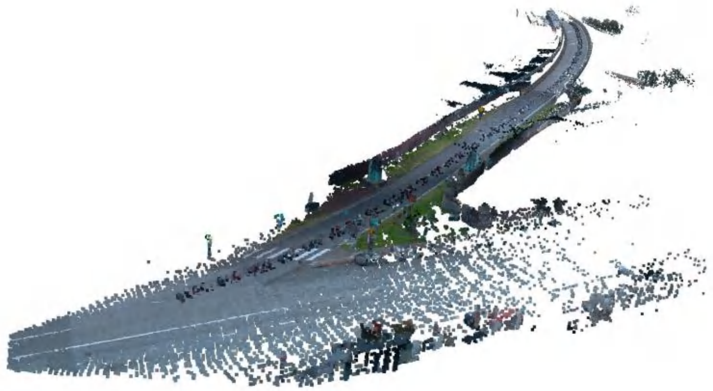

LiDAR

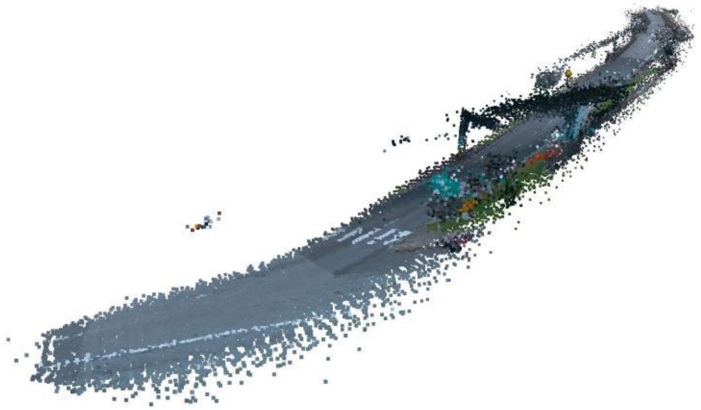

DROID-SLAM

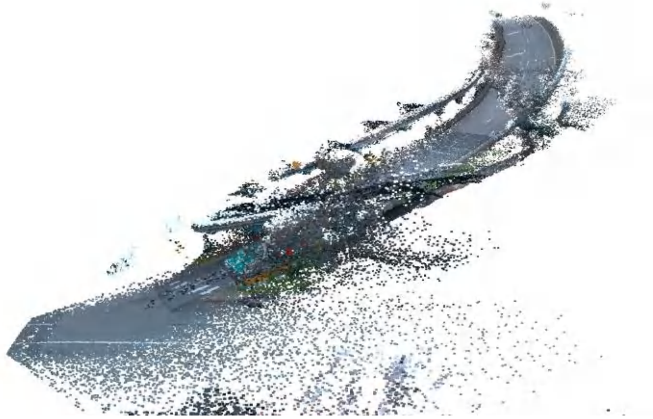

MASt3R-SLAM

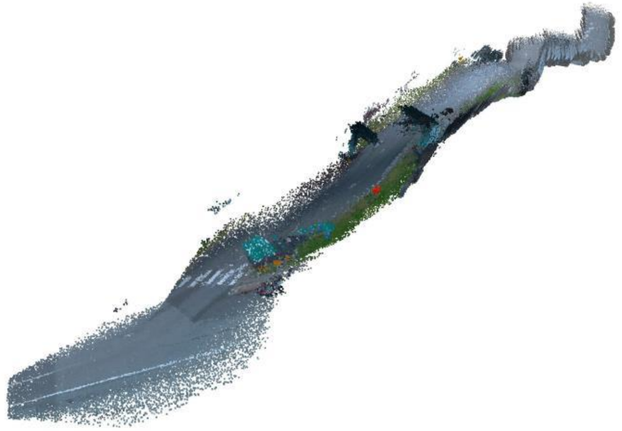

CUT3R

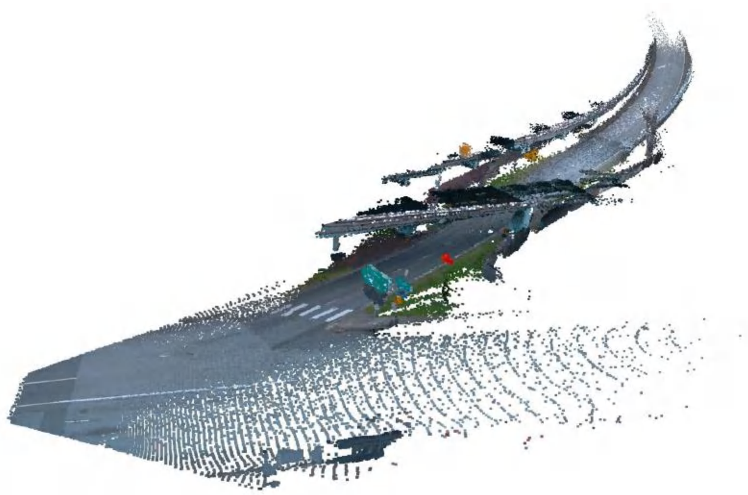

VGGT-Long

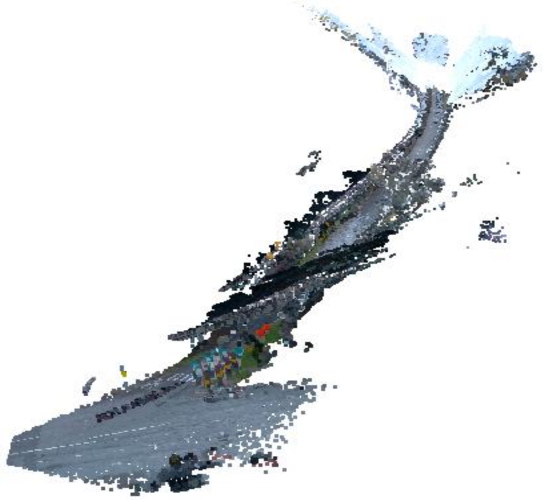

VGGT-SLAM

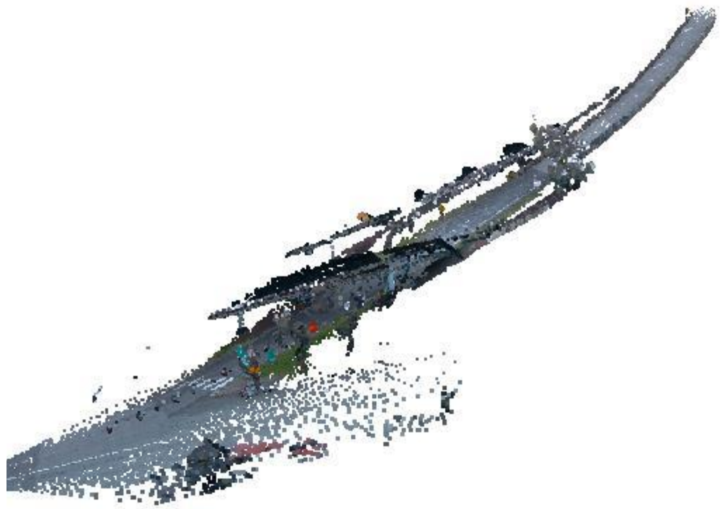

VGGT-Motion

# Segment-405841035 (85.743 m)

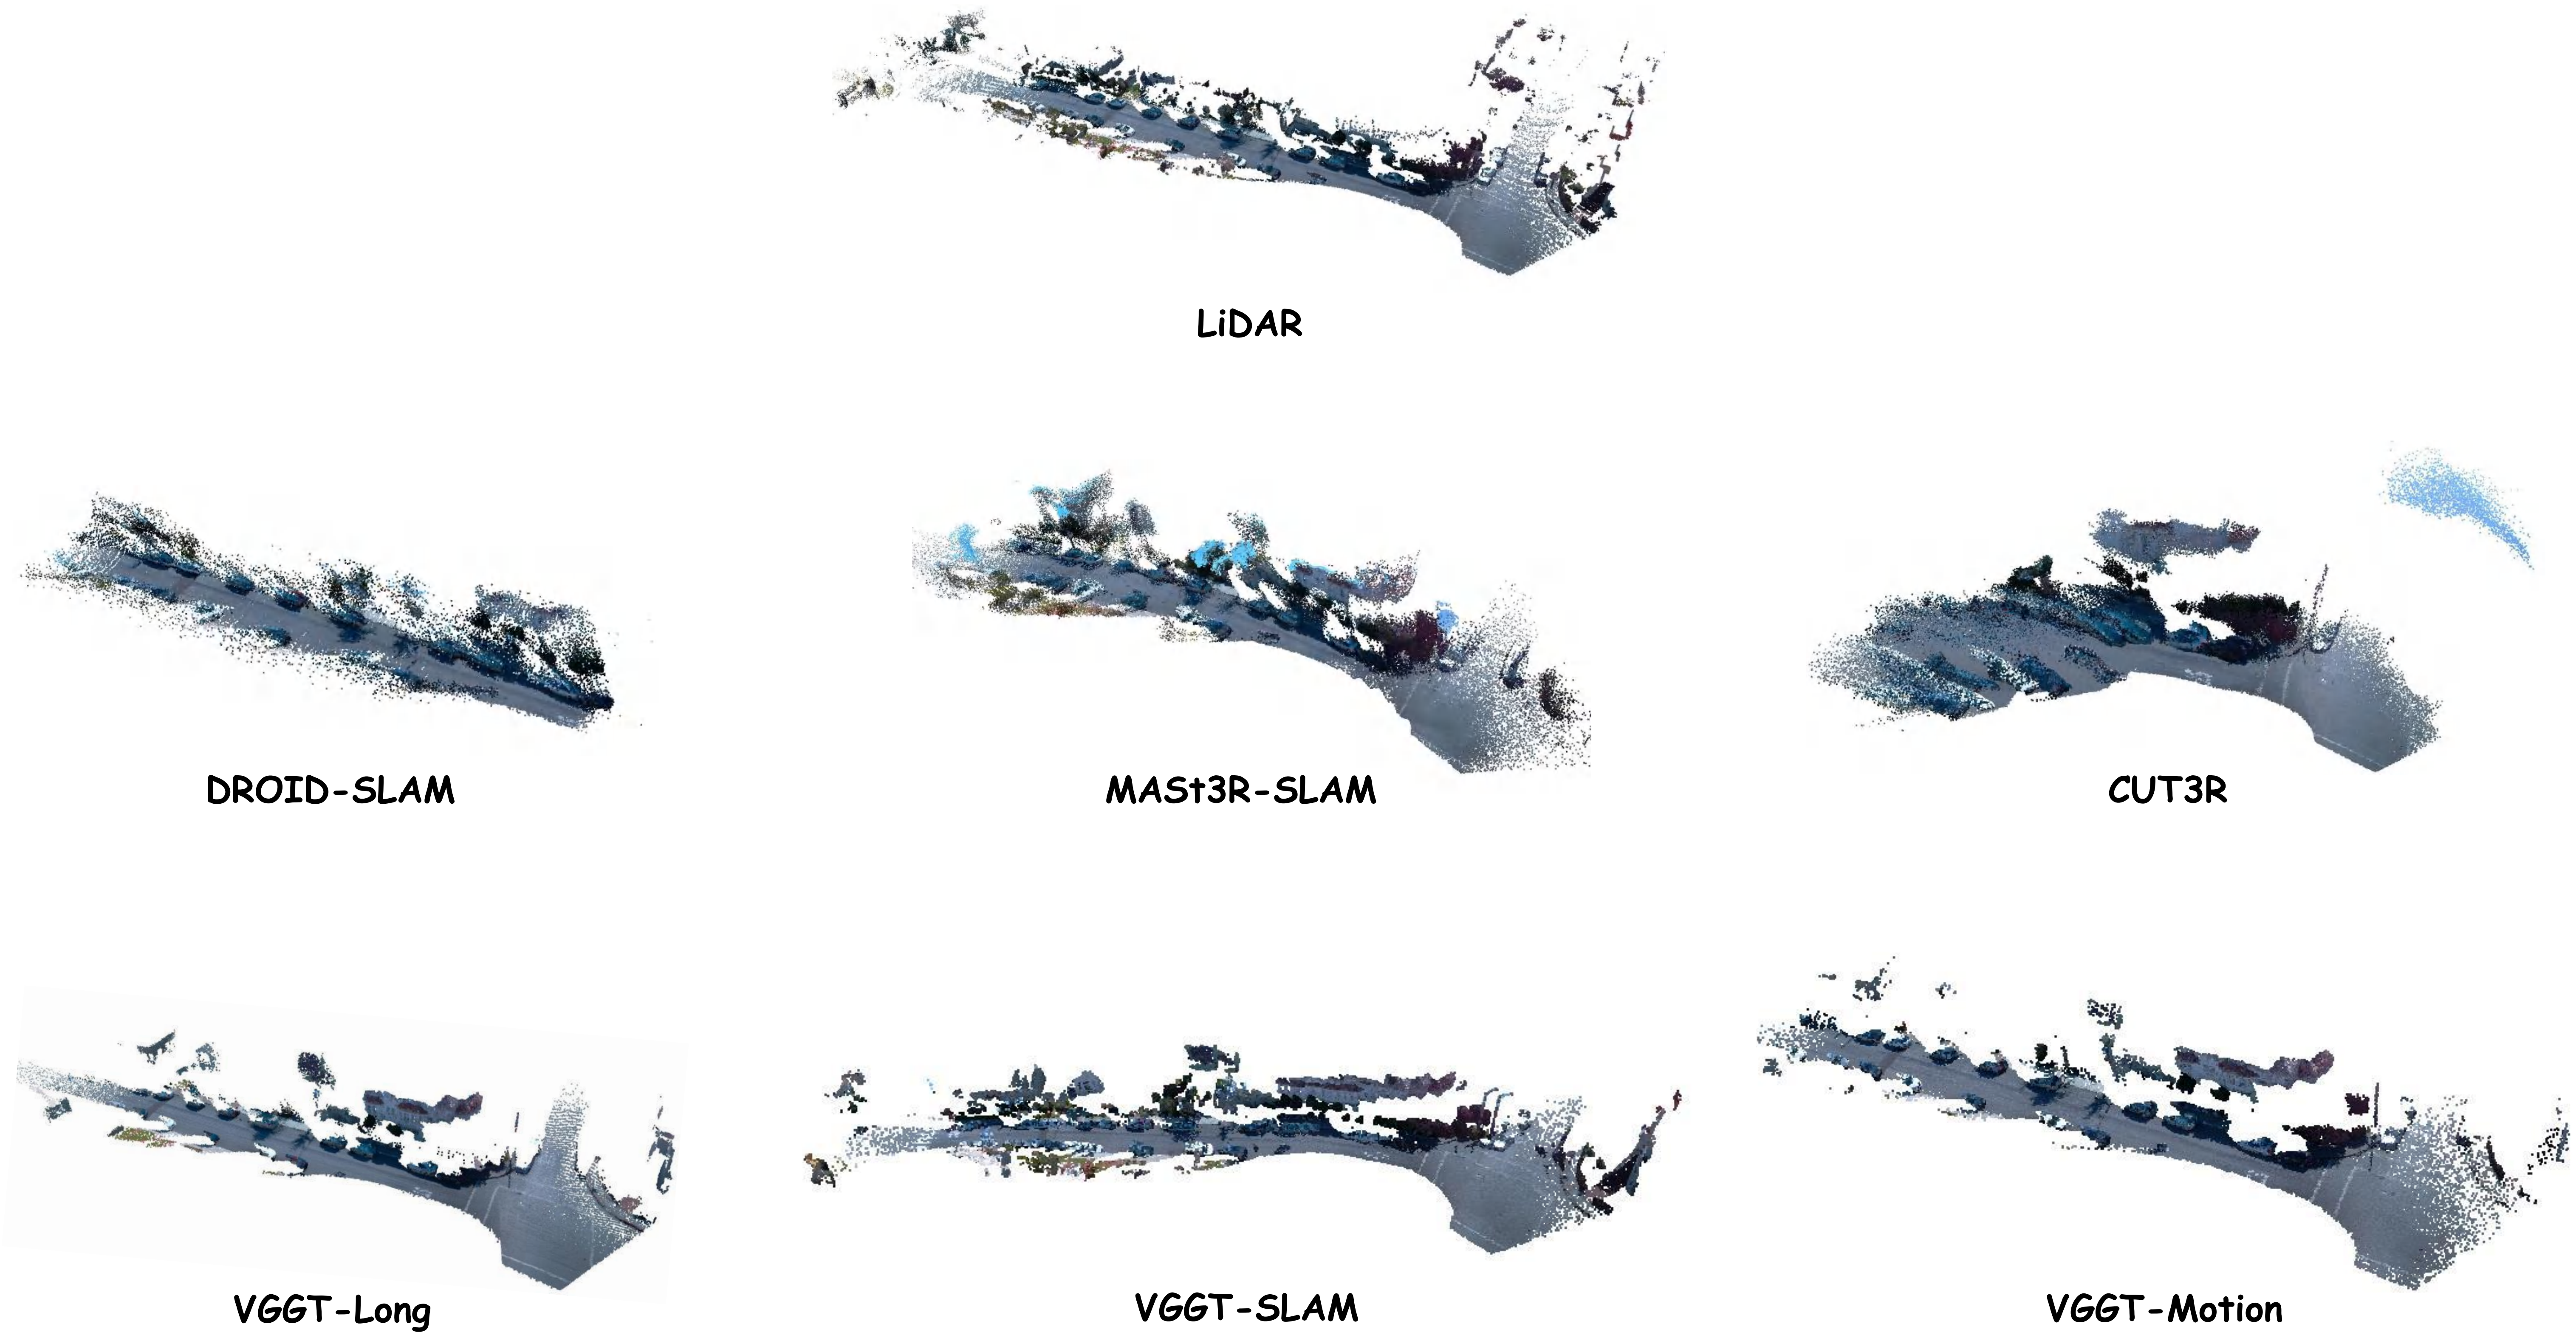

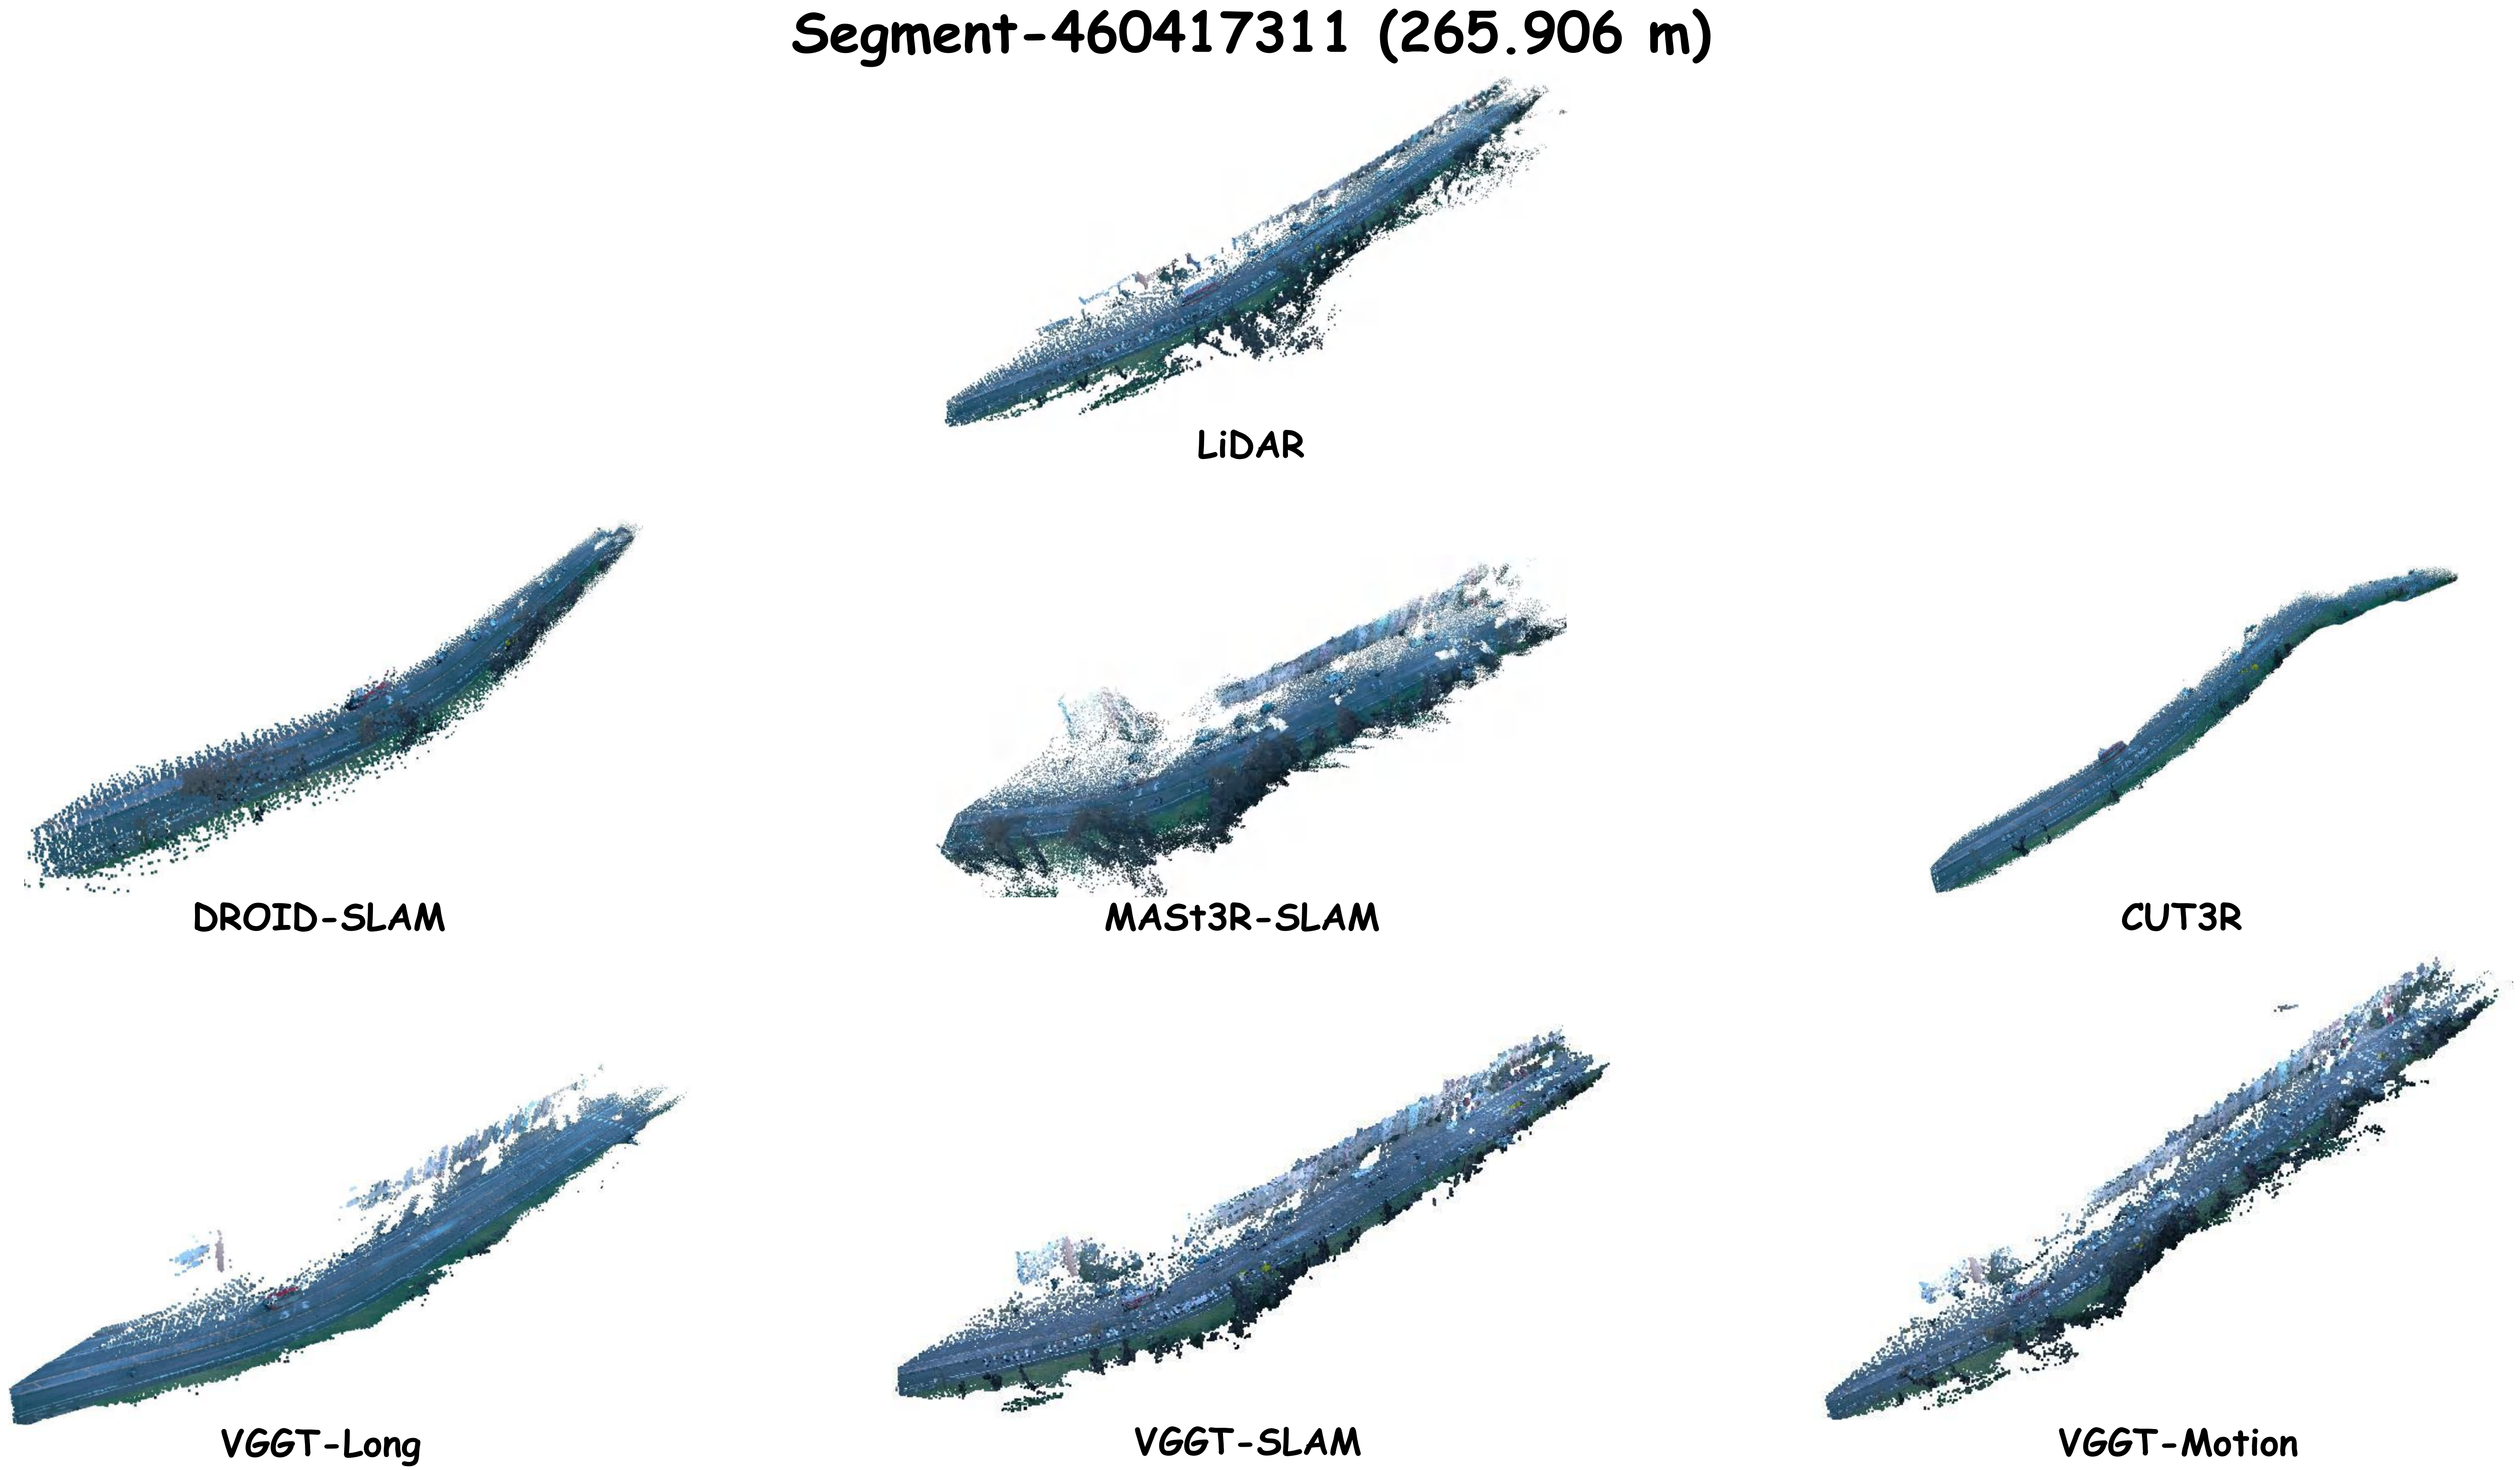
Segment-460417311 (265.906 m)
LiDAR
DROID-SLAM
MASt3R-SLAM
CUT3R
VGGT-Long
VGGT-SLAM
VGGT-Motion

Segment-520018670 (134.552 m)

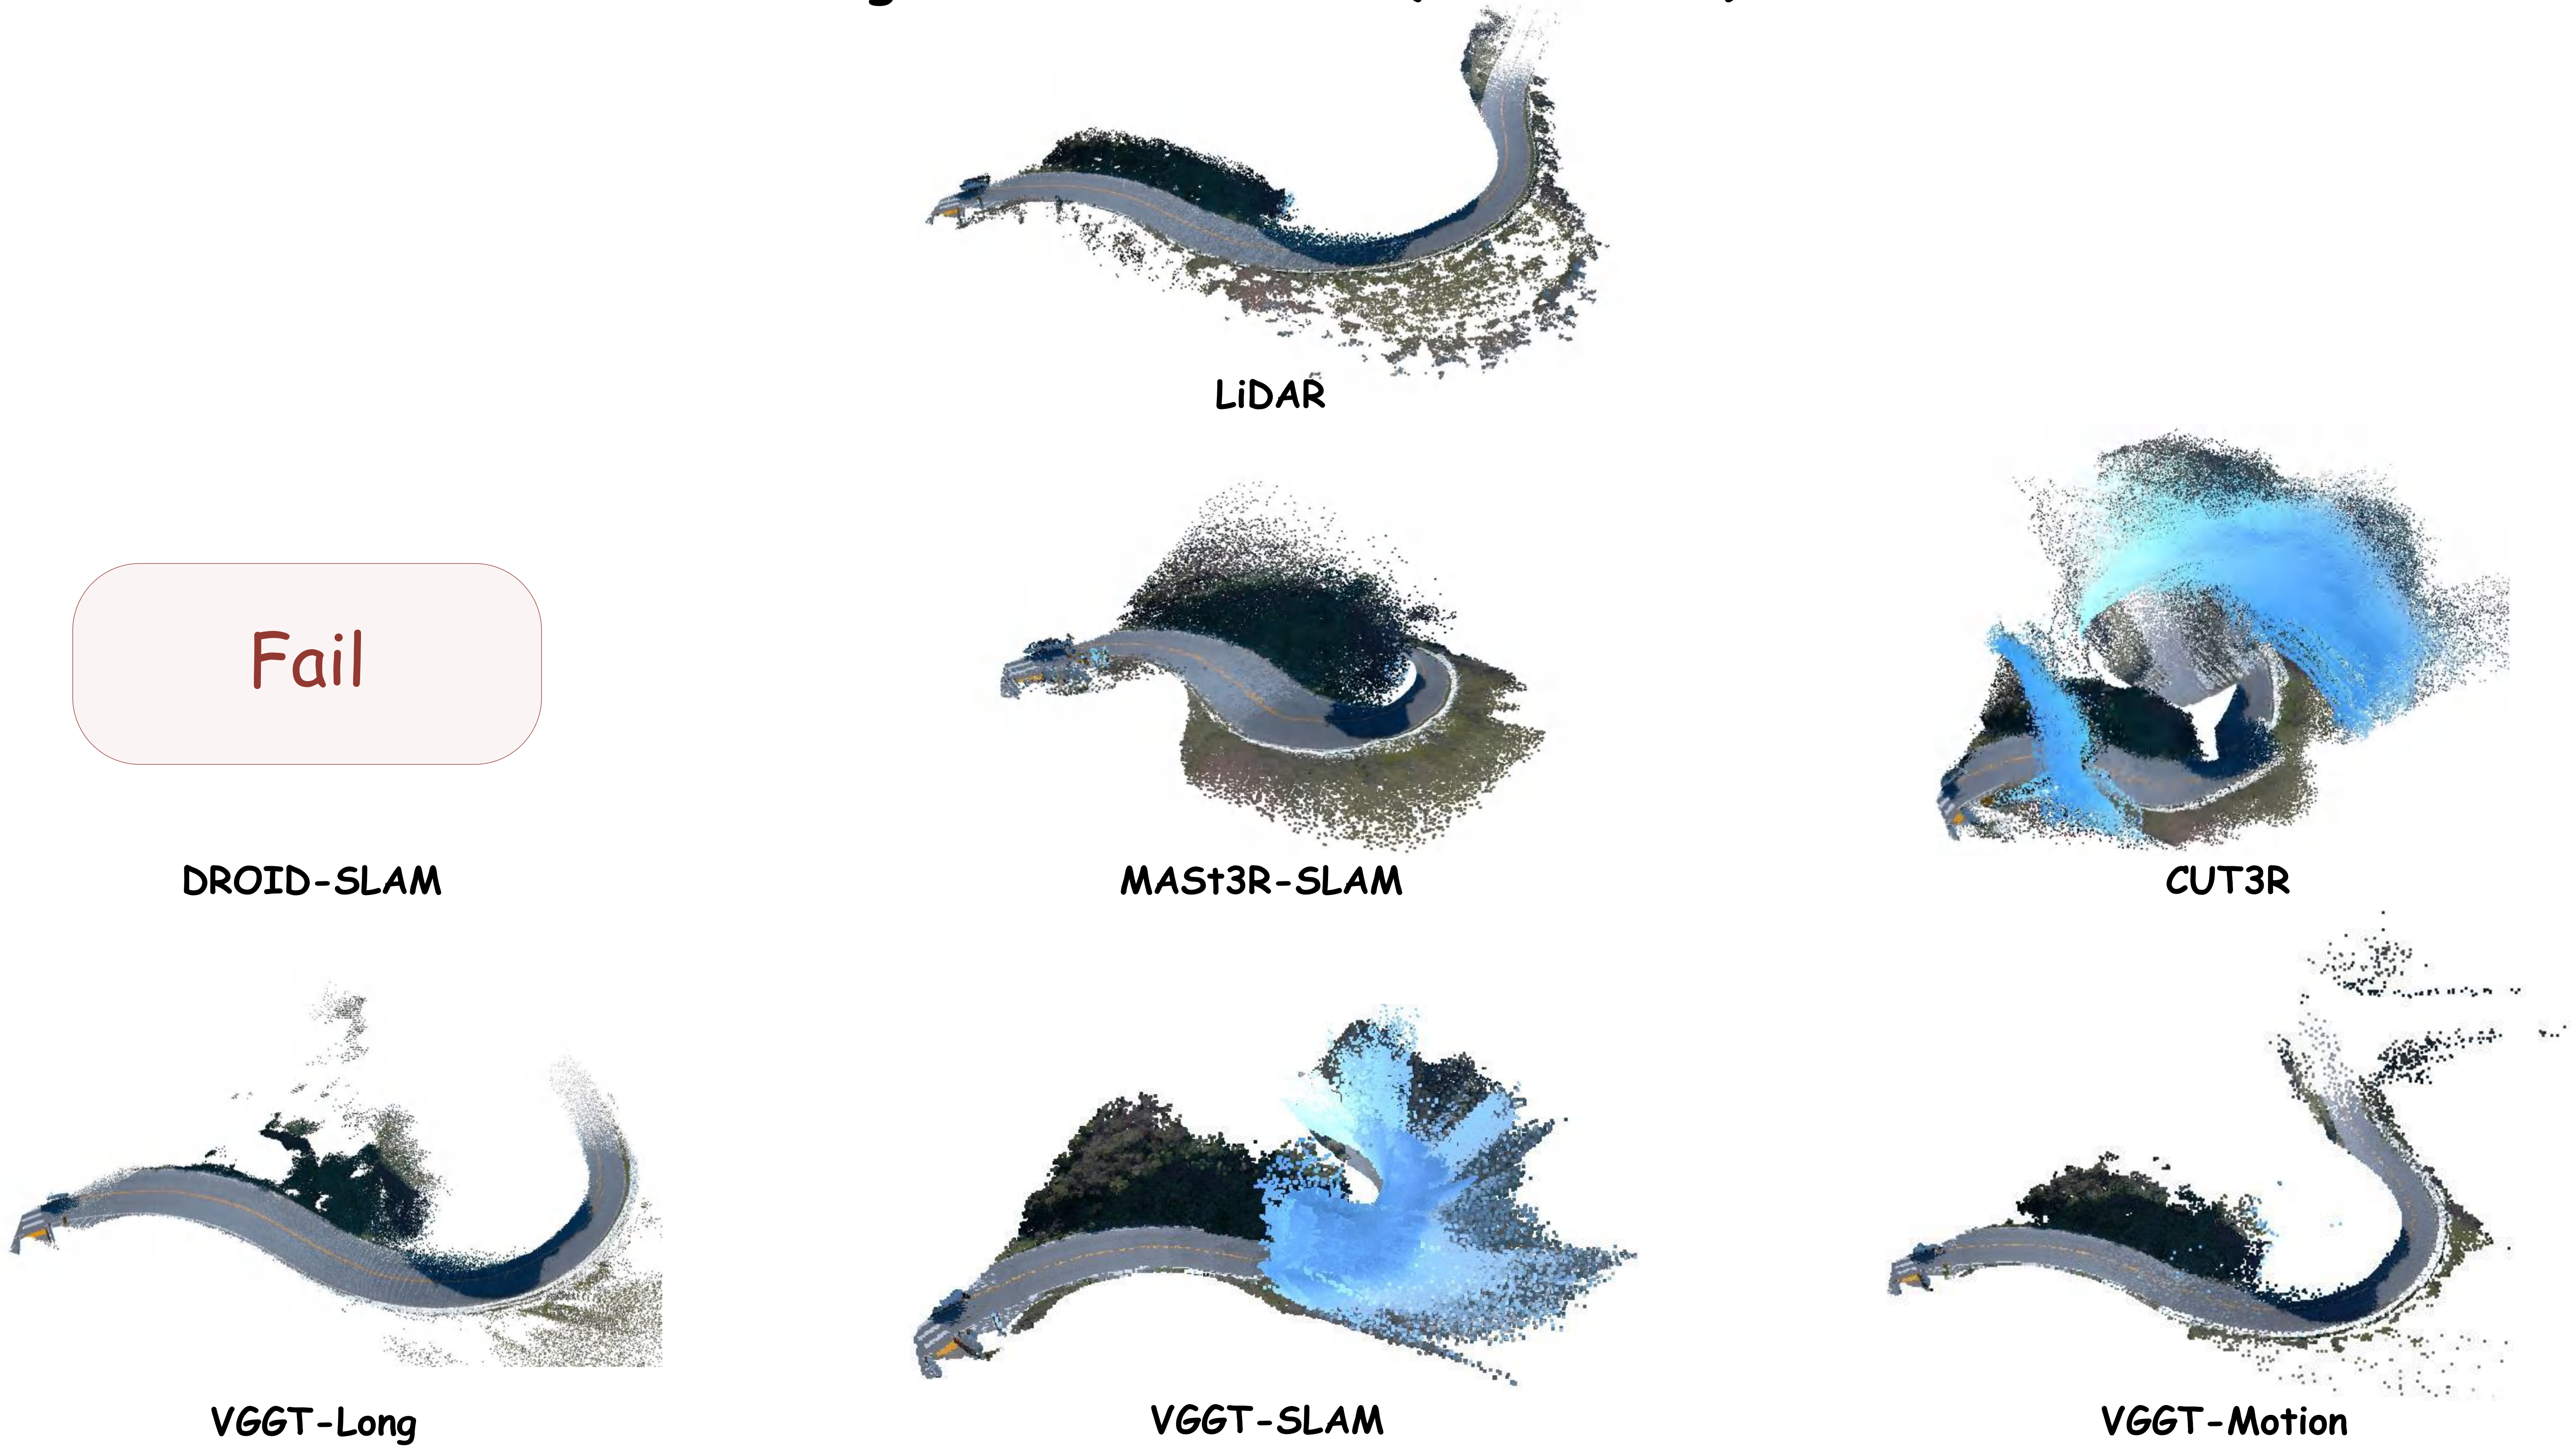

# Segment-610454533 (62.739 m)

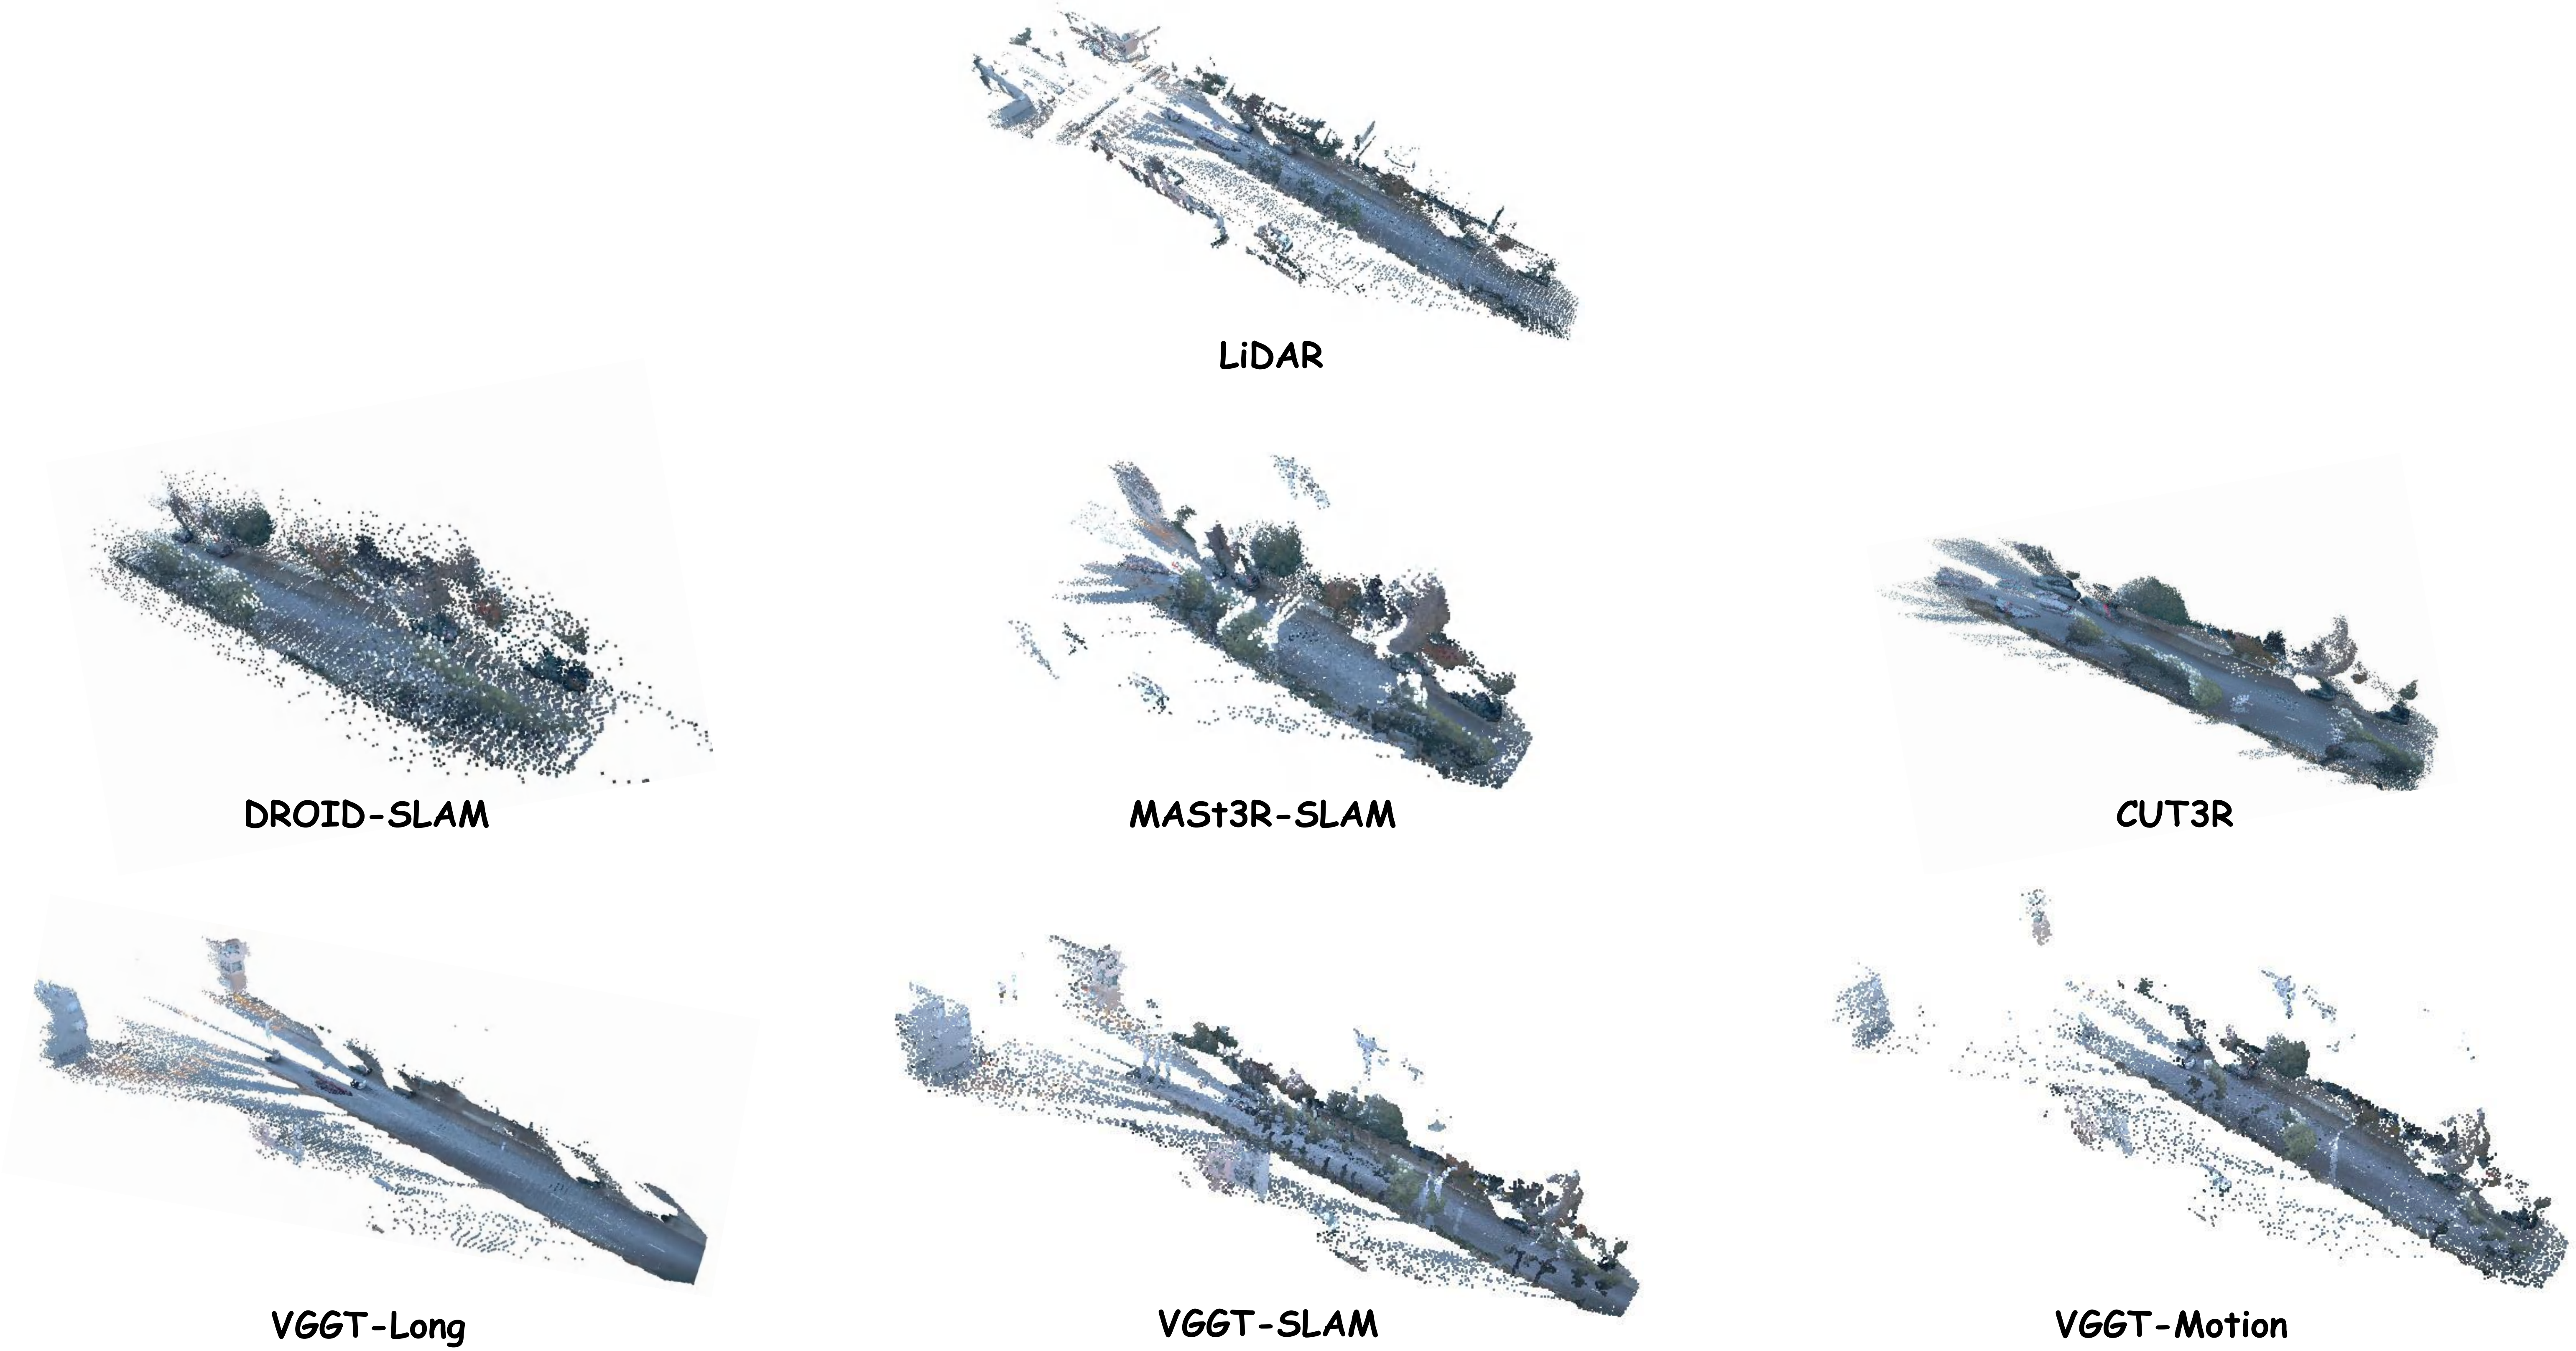

Supplement: Supplementary file 2 [file waymo-point.pdf]
