# Supplementary material for: VGGT-Motion: Motion-Aware Calibration-Free Monocular SLAM for Long-Range Consistency
Source: arXiv:2602.05508 source file (2026-02-05)

Ours(vggt)

Ours(pi3)

Ours(da3)

Sequence -00

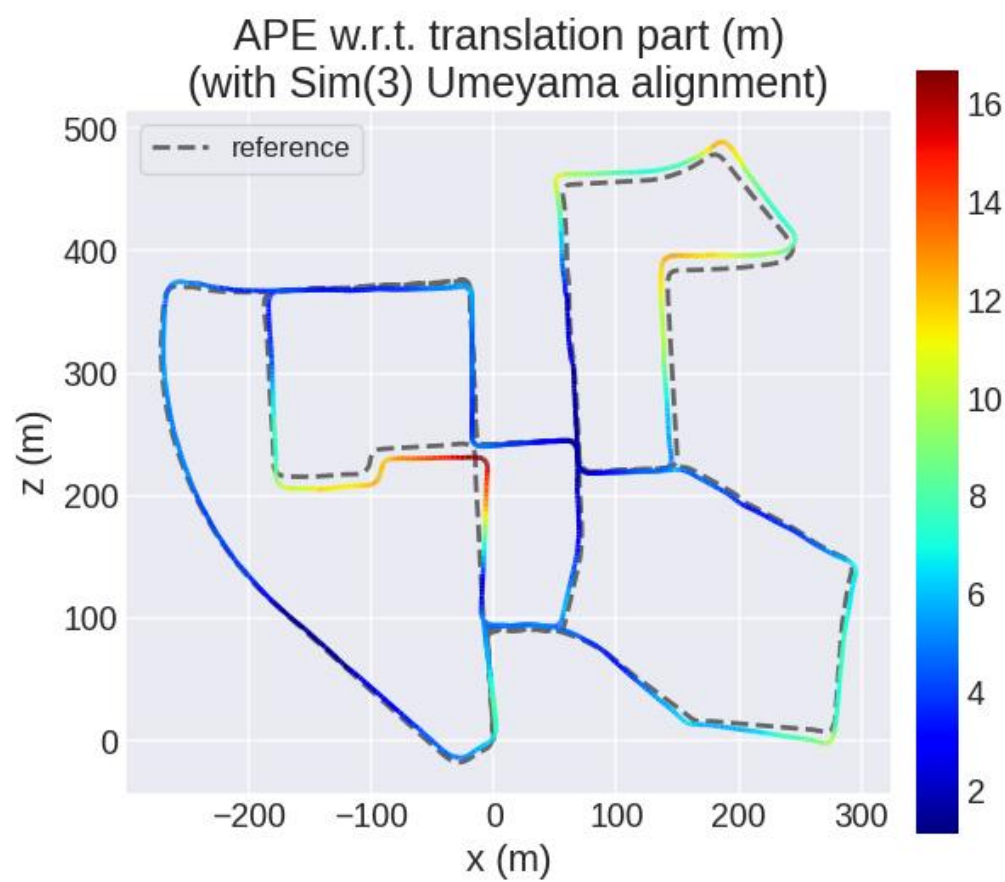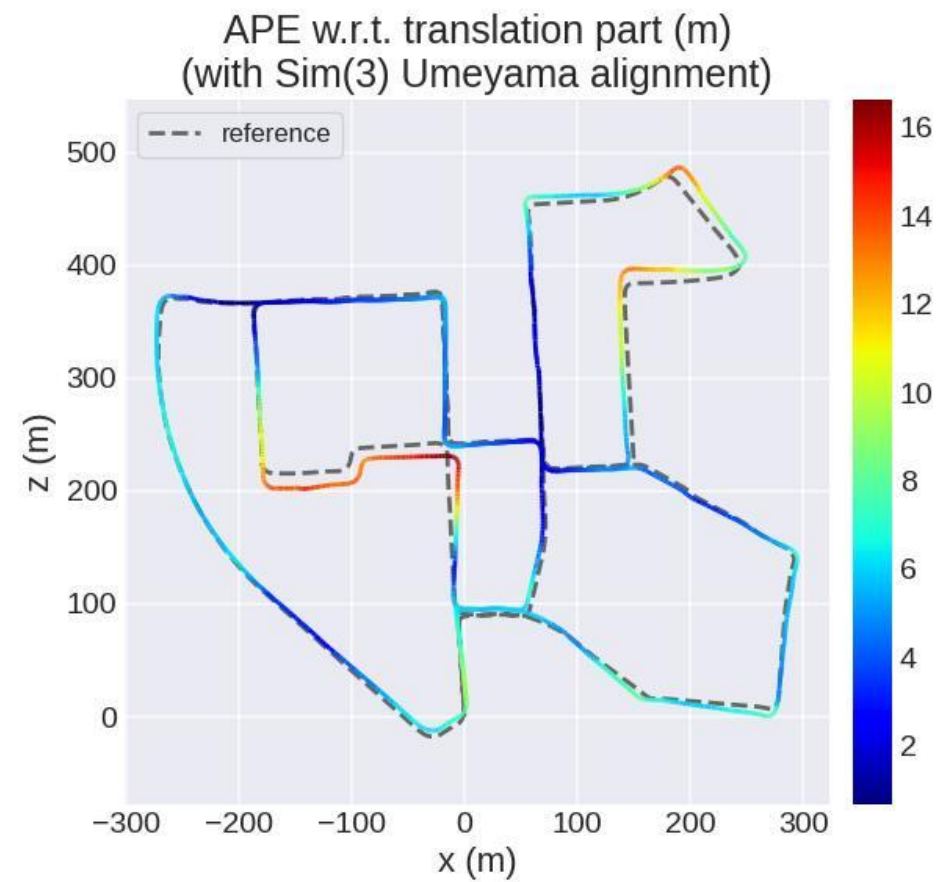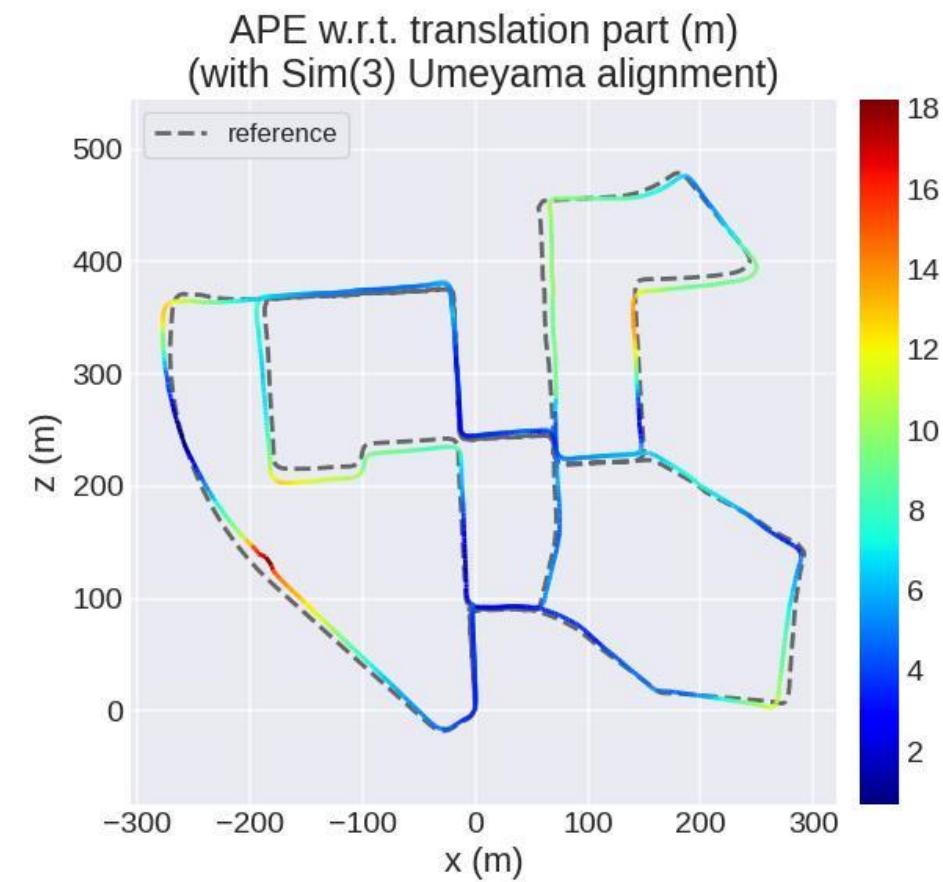

Sequence -05

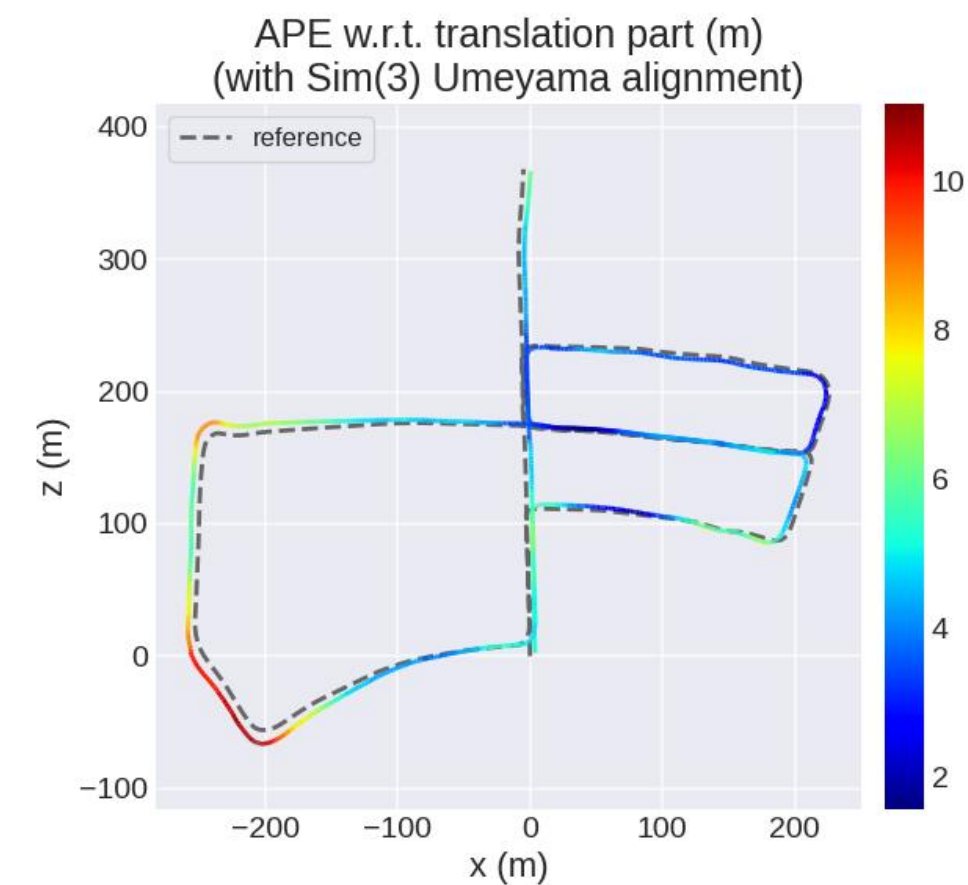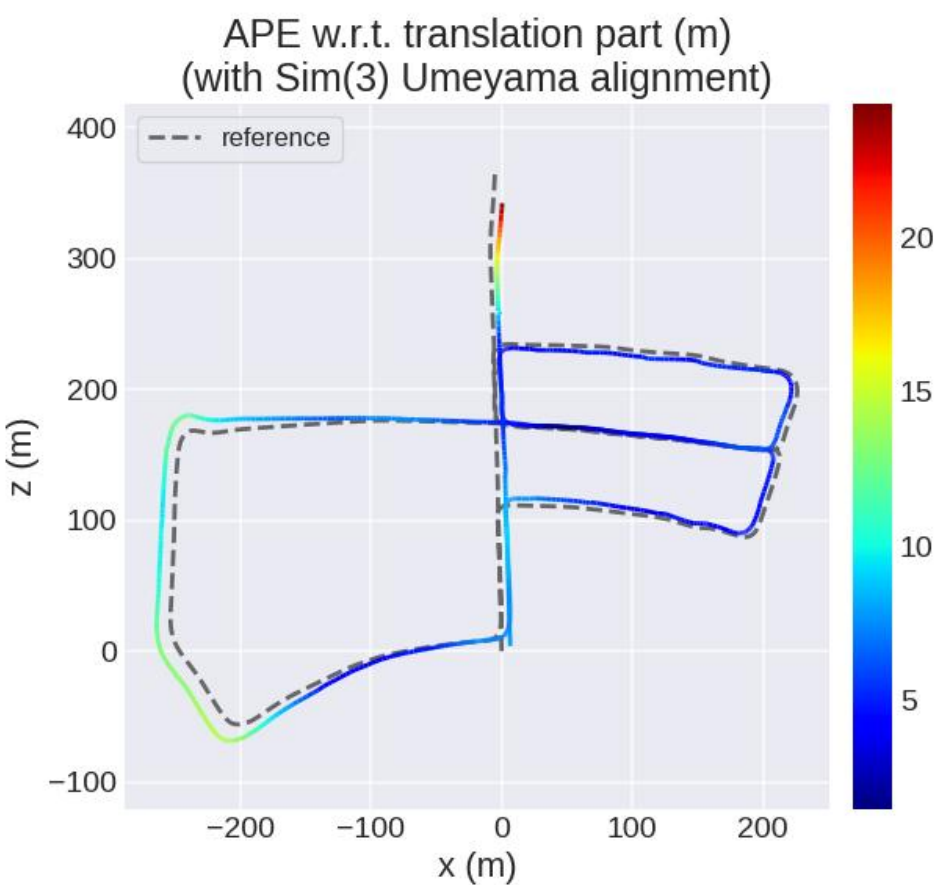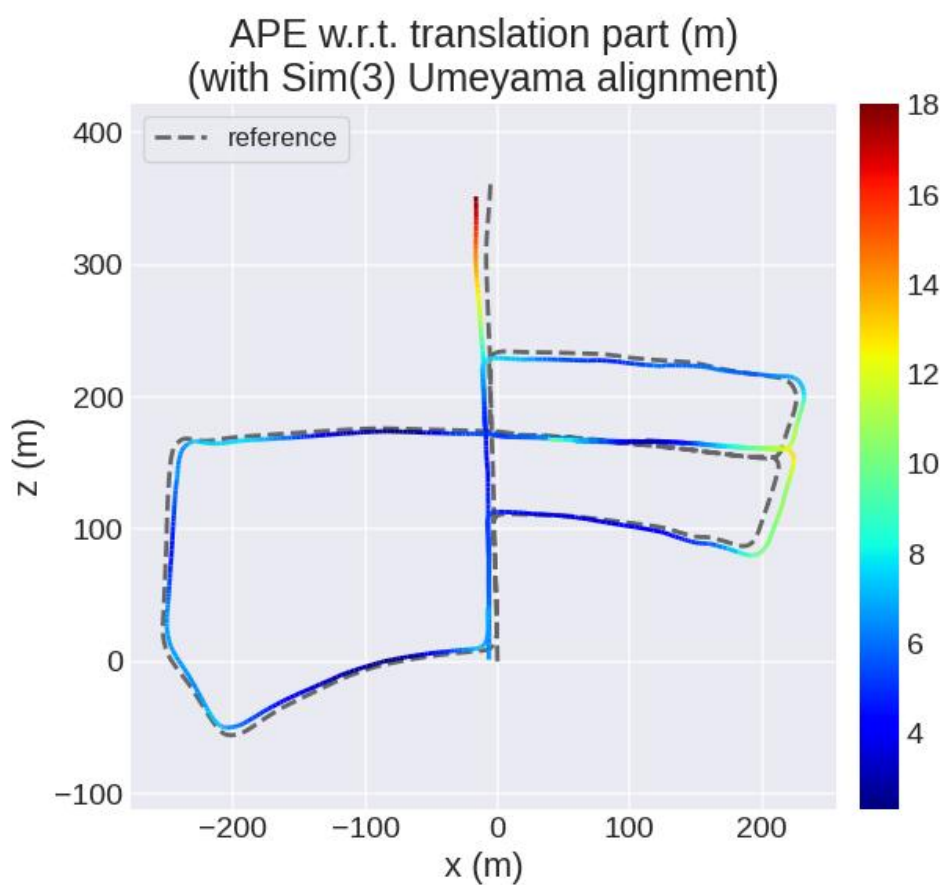

Segment-460417311

Ours(vggt)

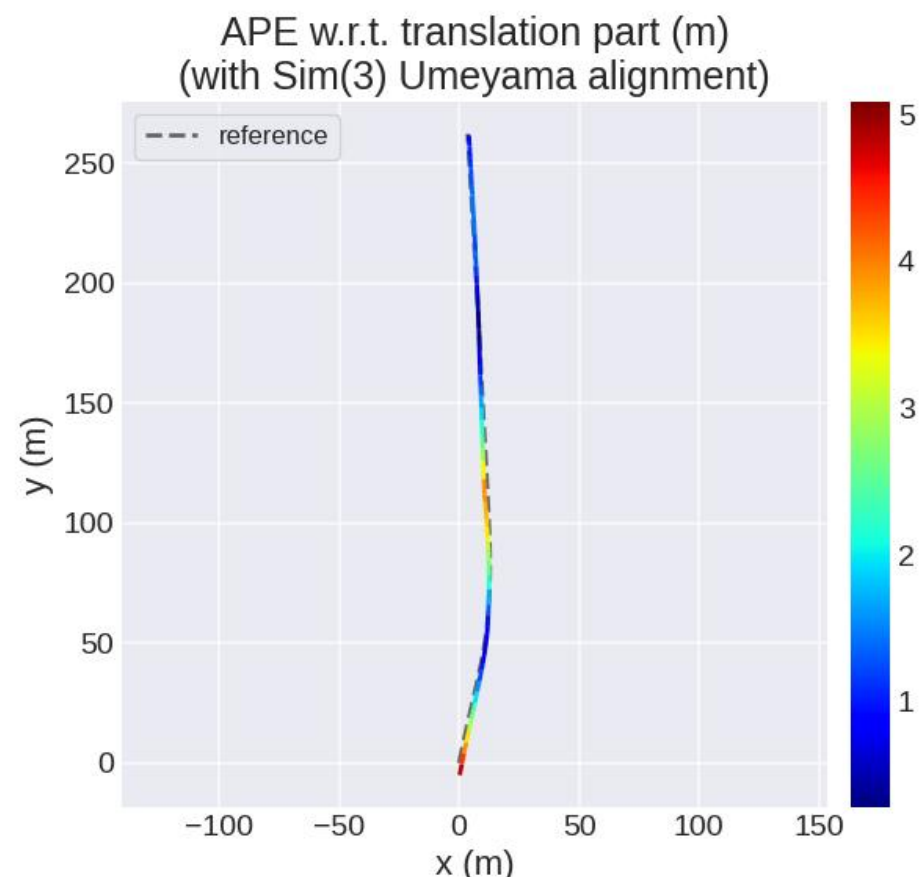

Ours(pi3)

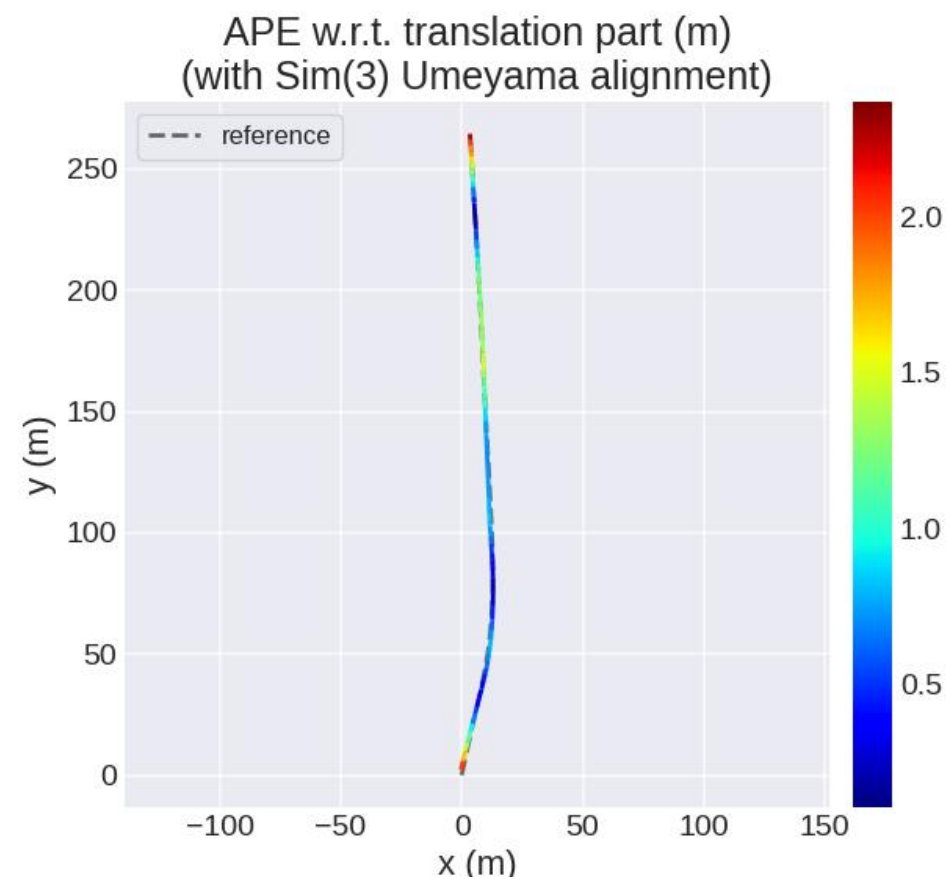

Ours(da3)

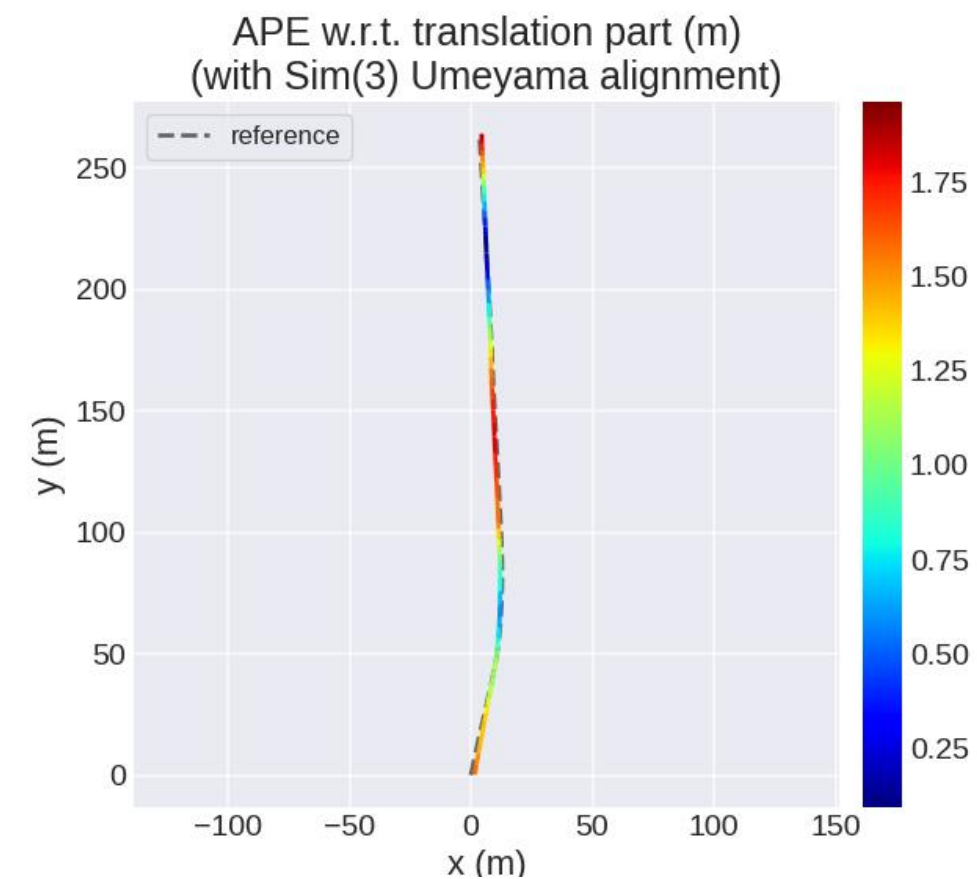

Segment-520018670

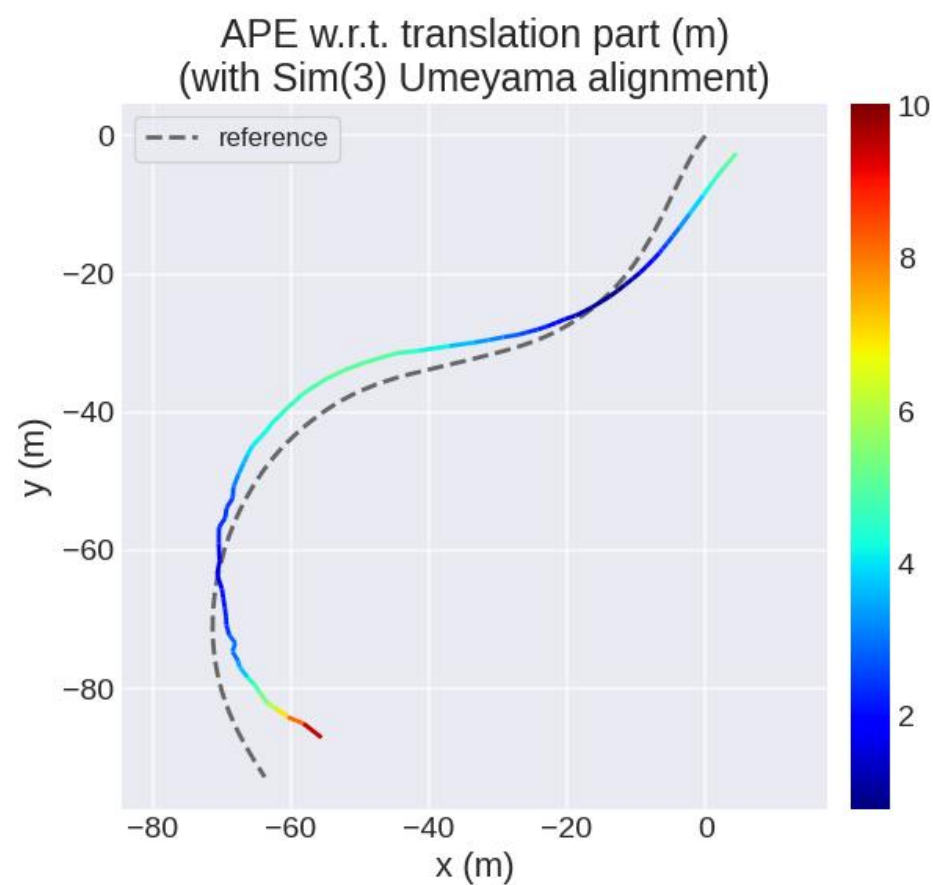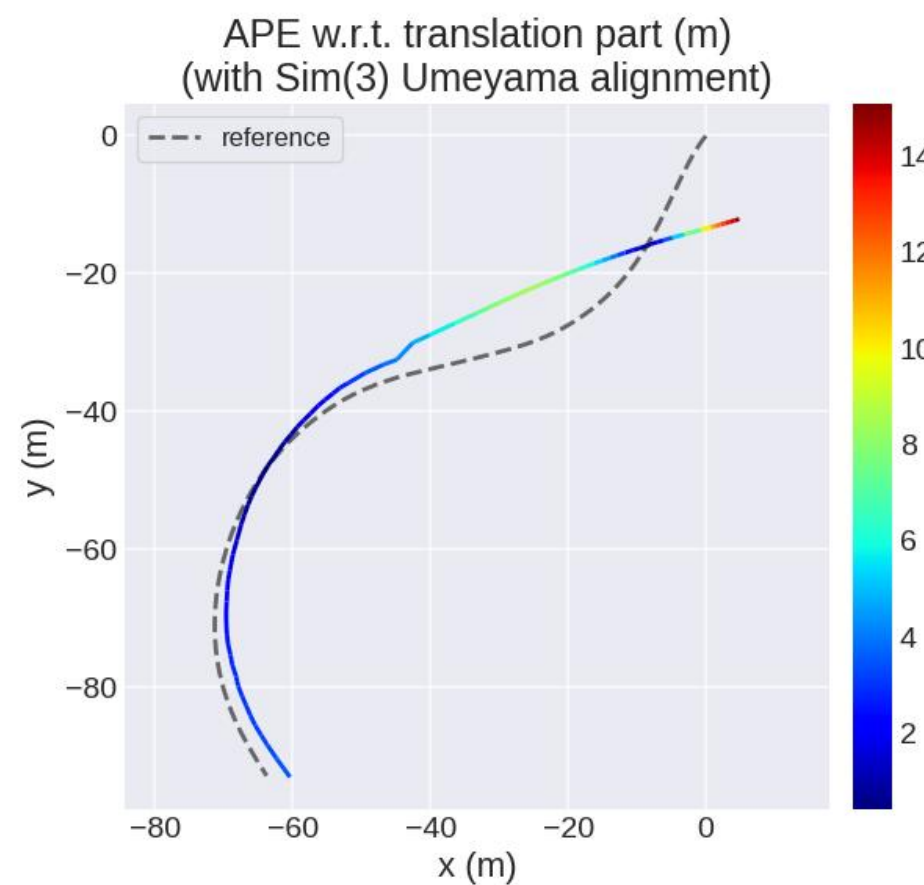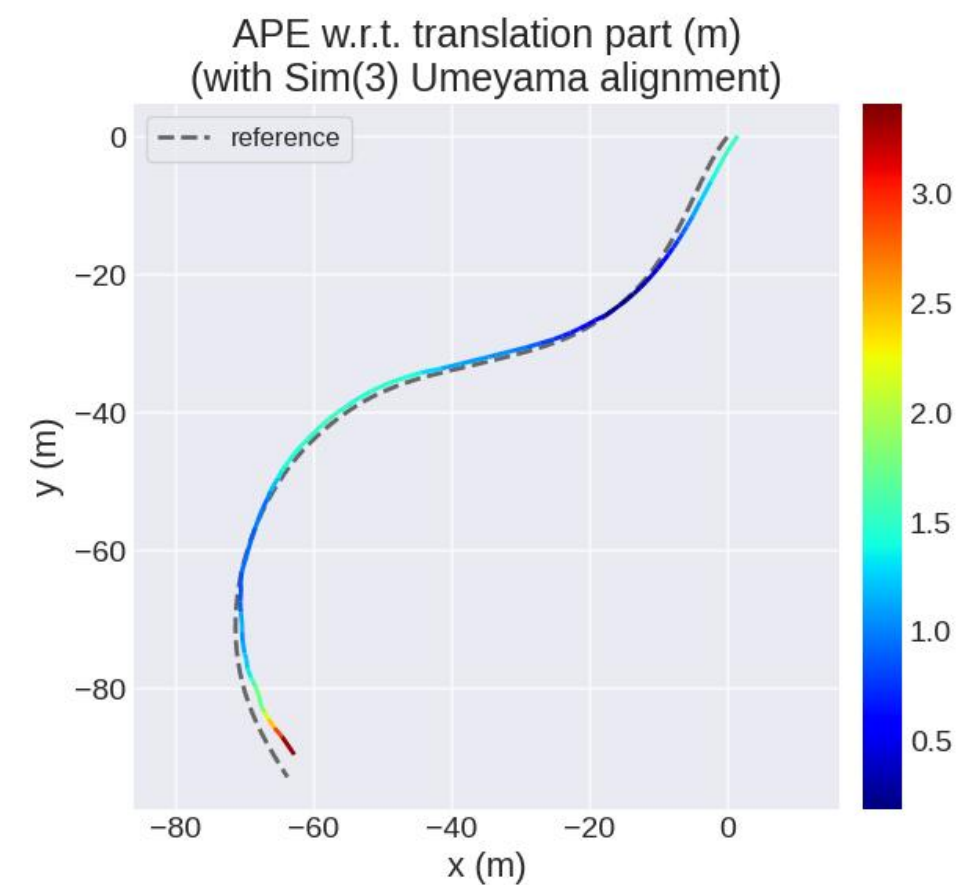

# Sequence-00

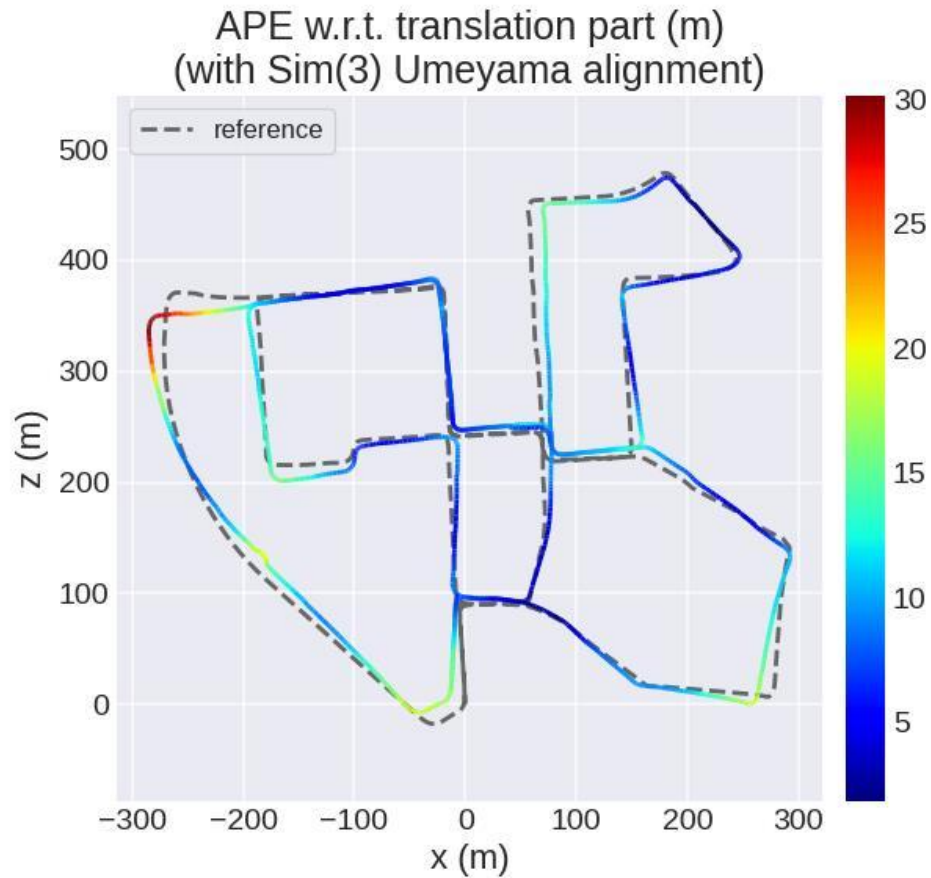

# Sequence-05

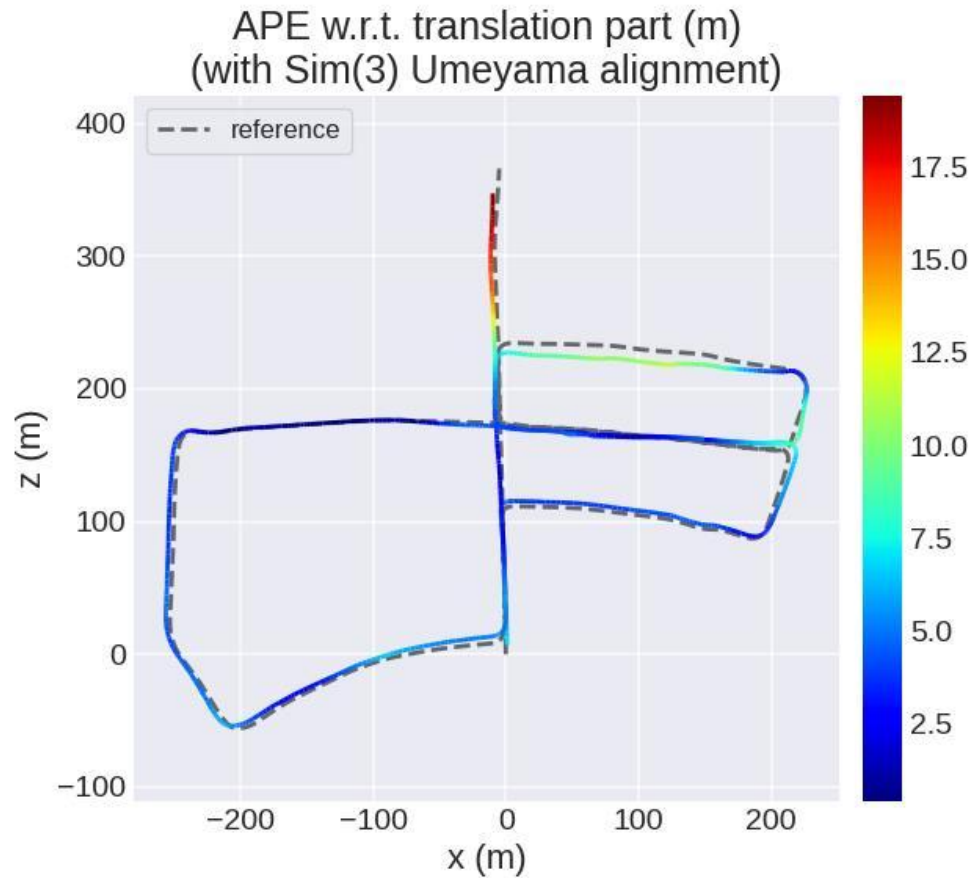

Supplement: Supplementary file 3 [file b1.pdf]
