# Supplementary material for: VGGT-Motion: Motion-Aware Calibration-Free Monocular SLAM for Long-Range Consistency
Source: arXiv:2602.05508 source file (2026-02-05)

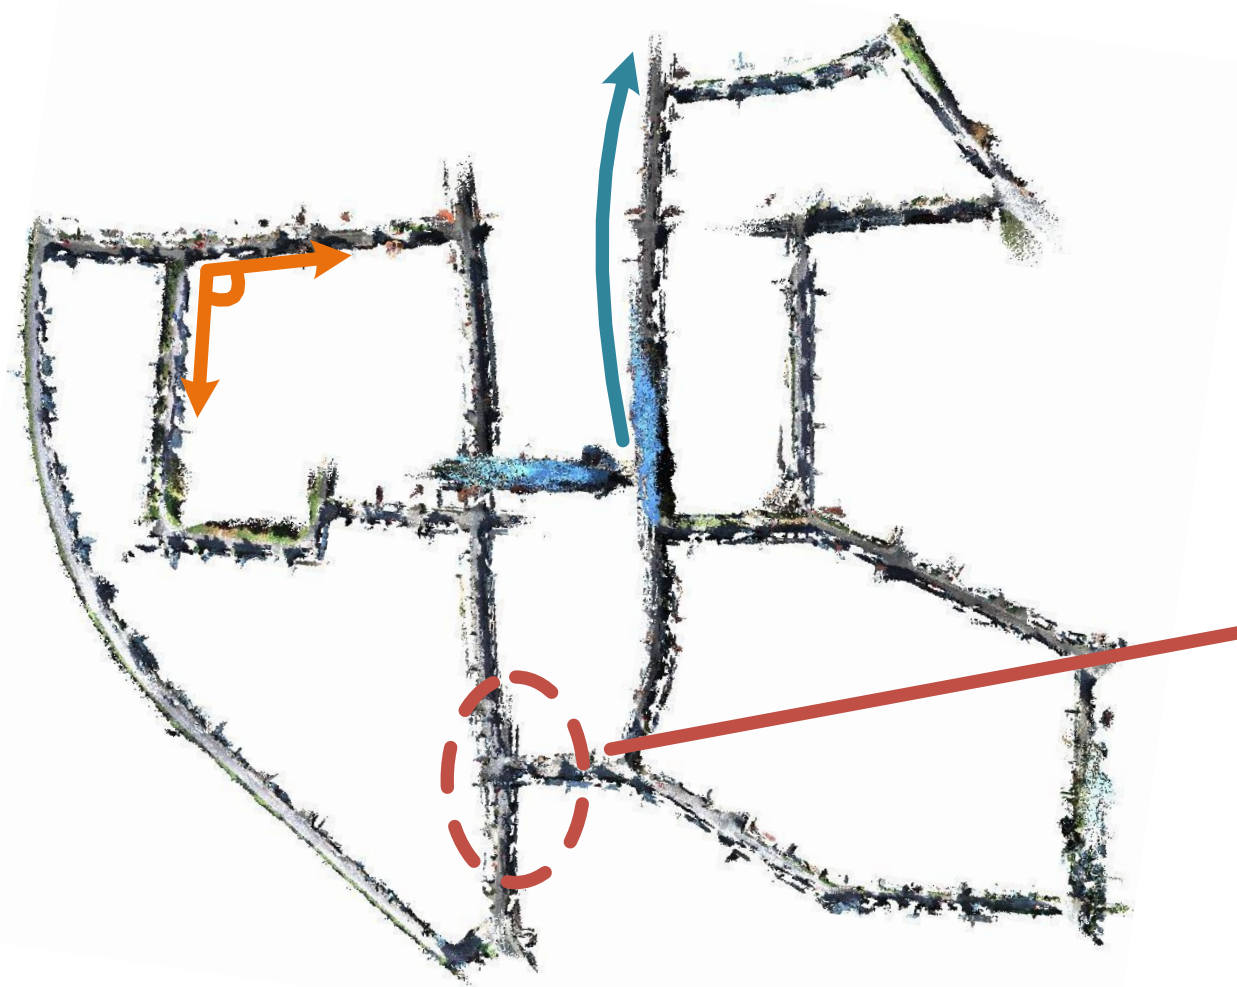

(a)VGGT-Long

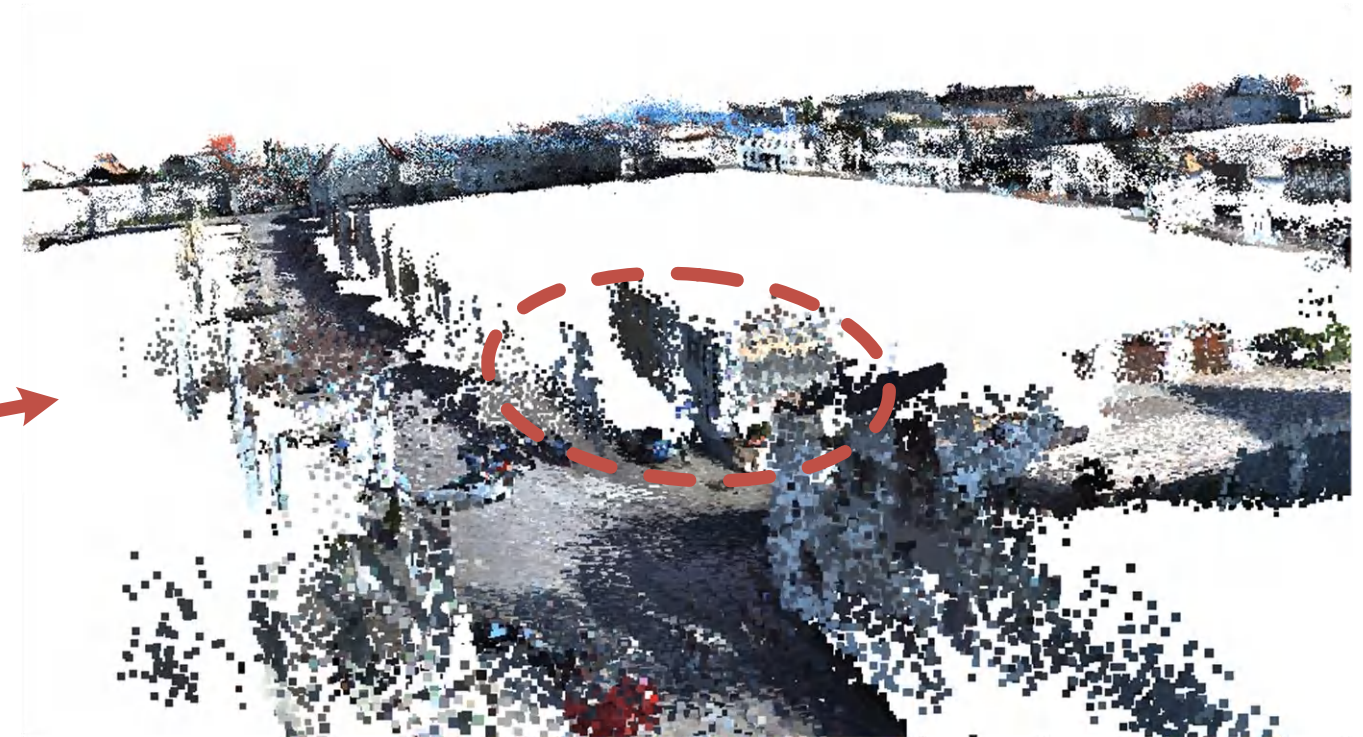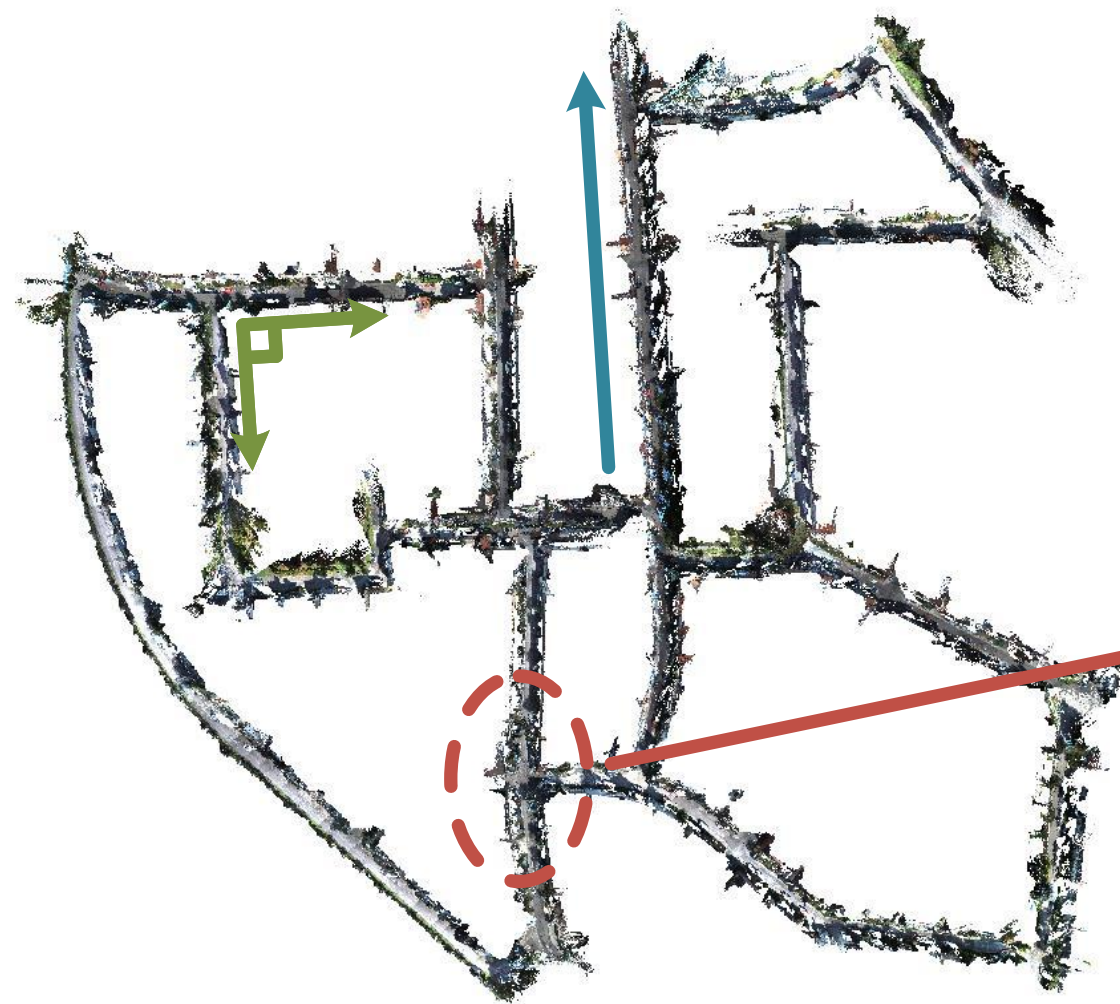

(b)VGGT-Motion

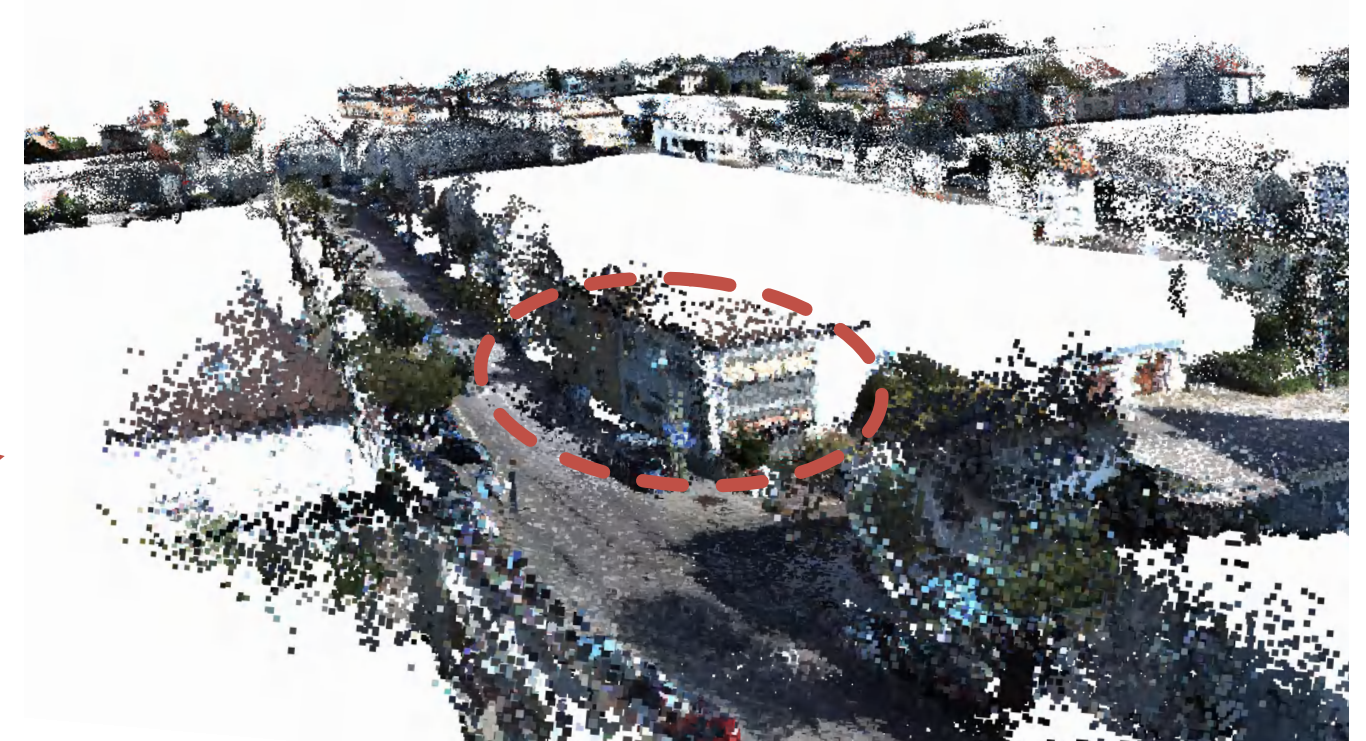



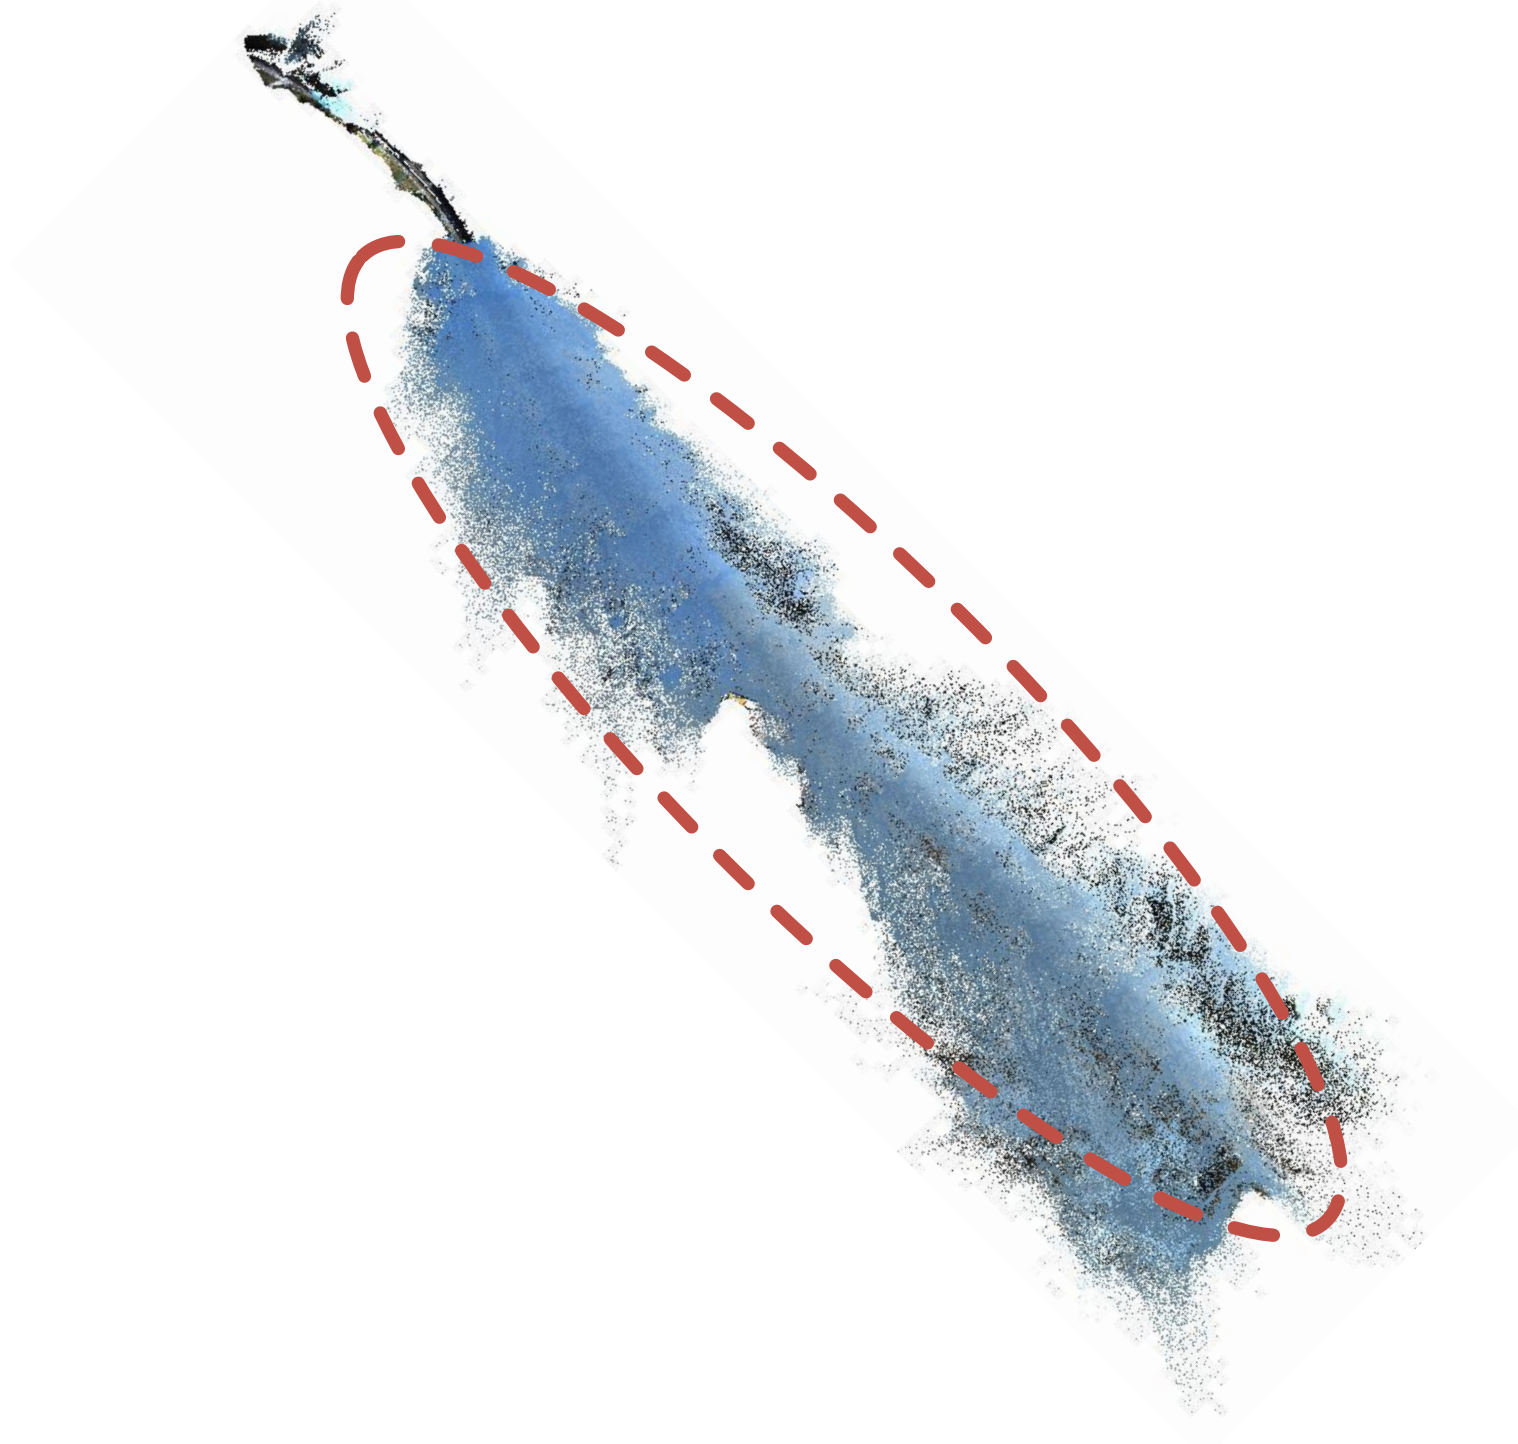

(a) VGGT-Long

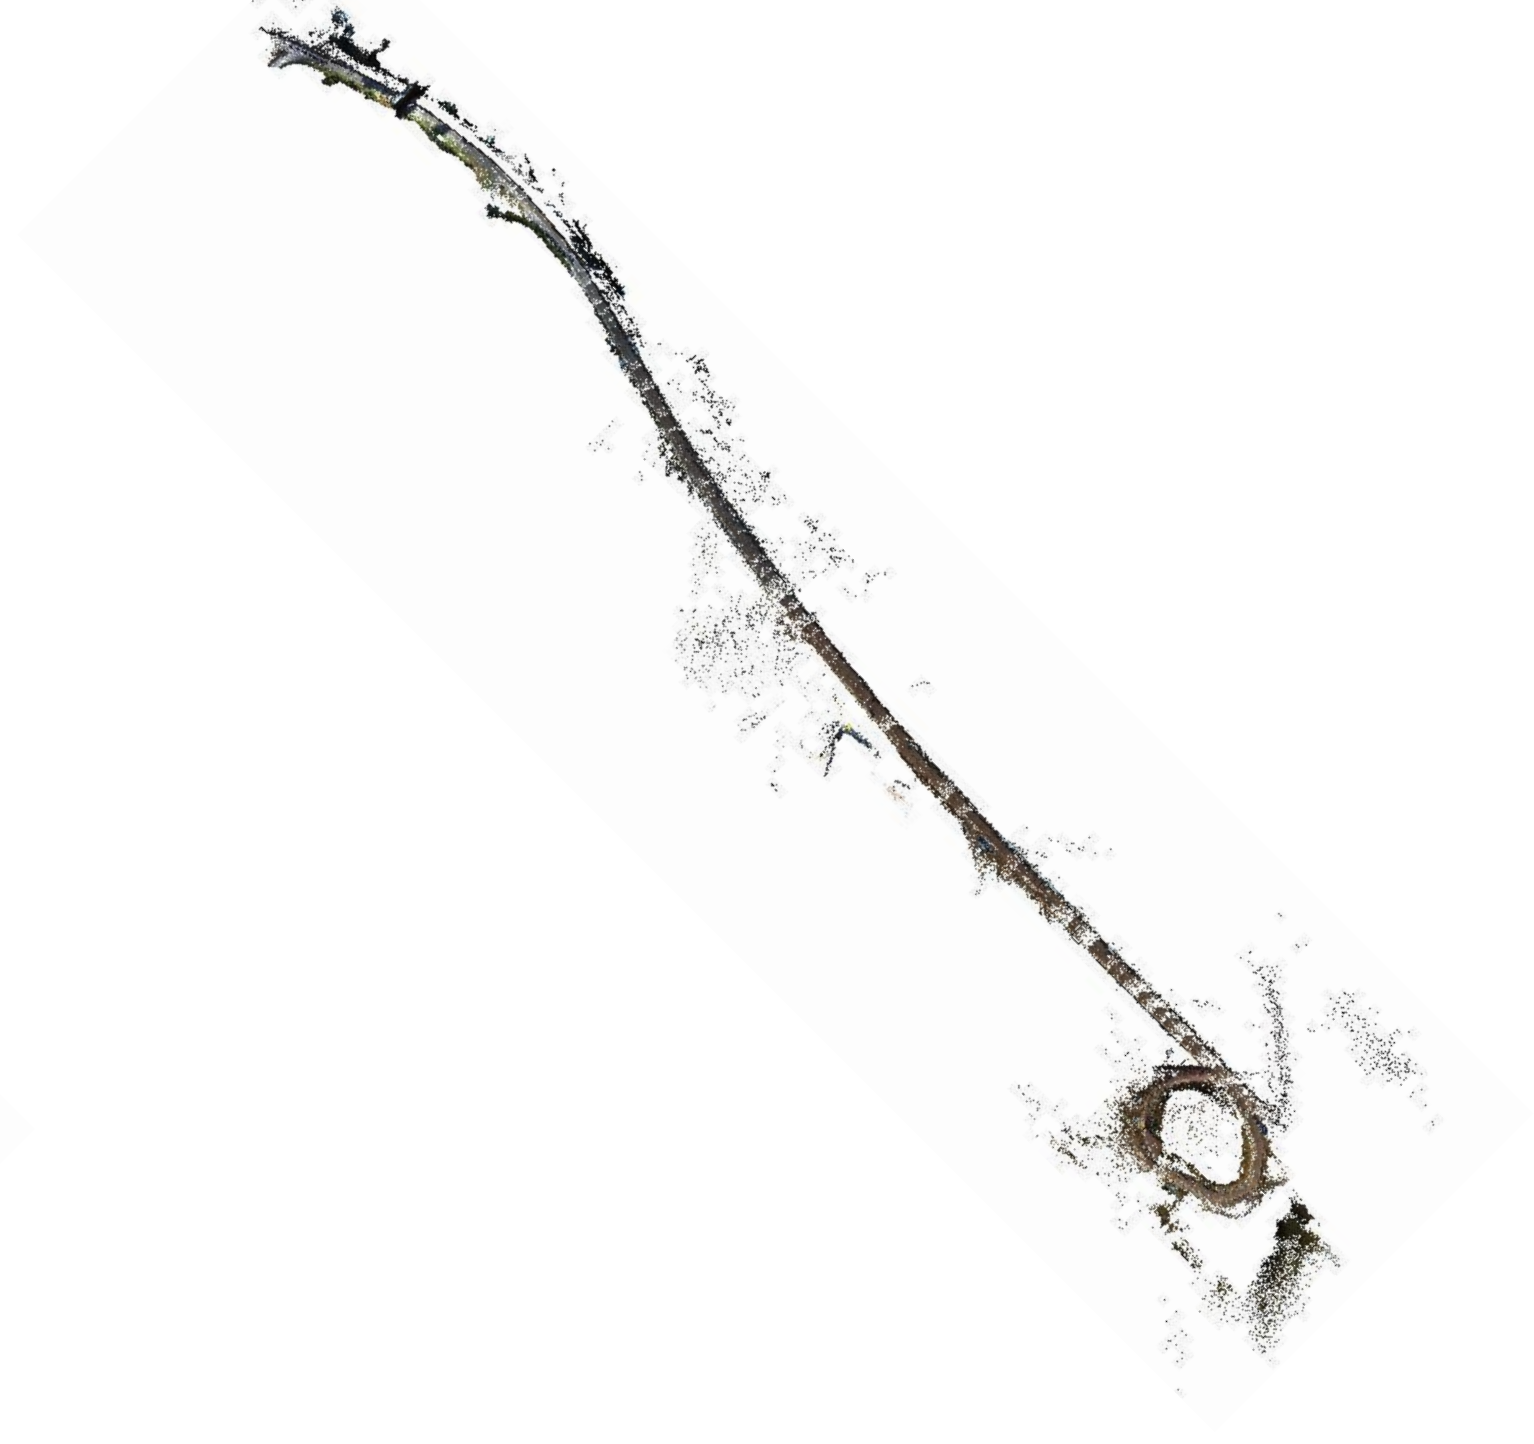

(b) VGGT-Motion



(a)VGGT-Long

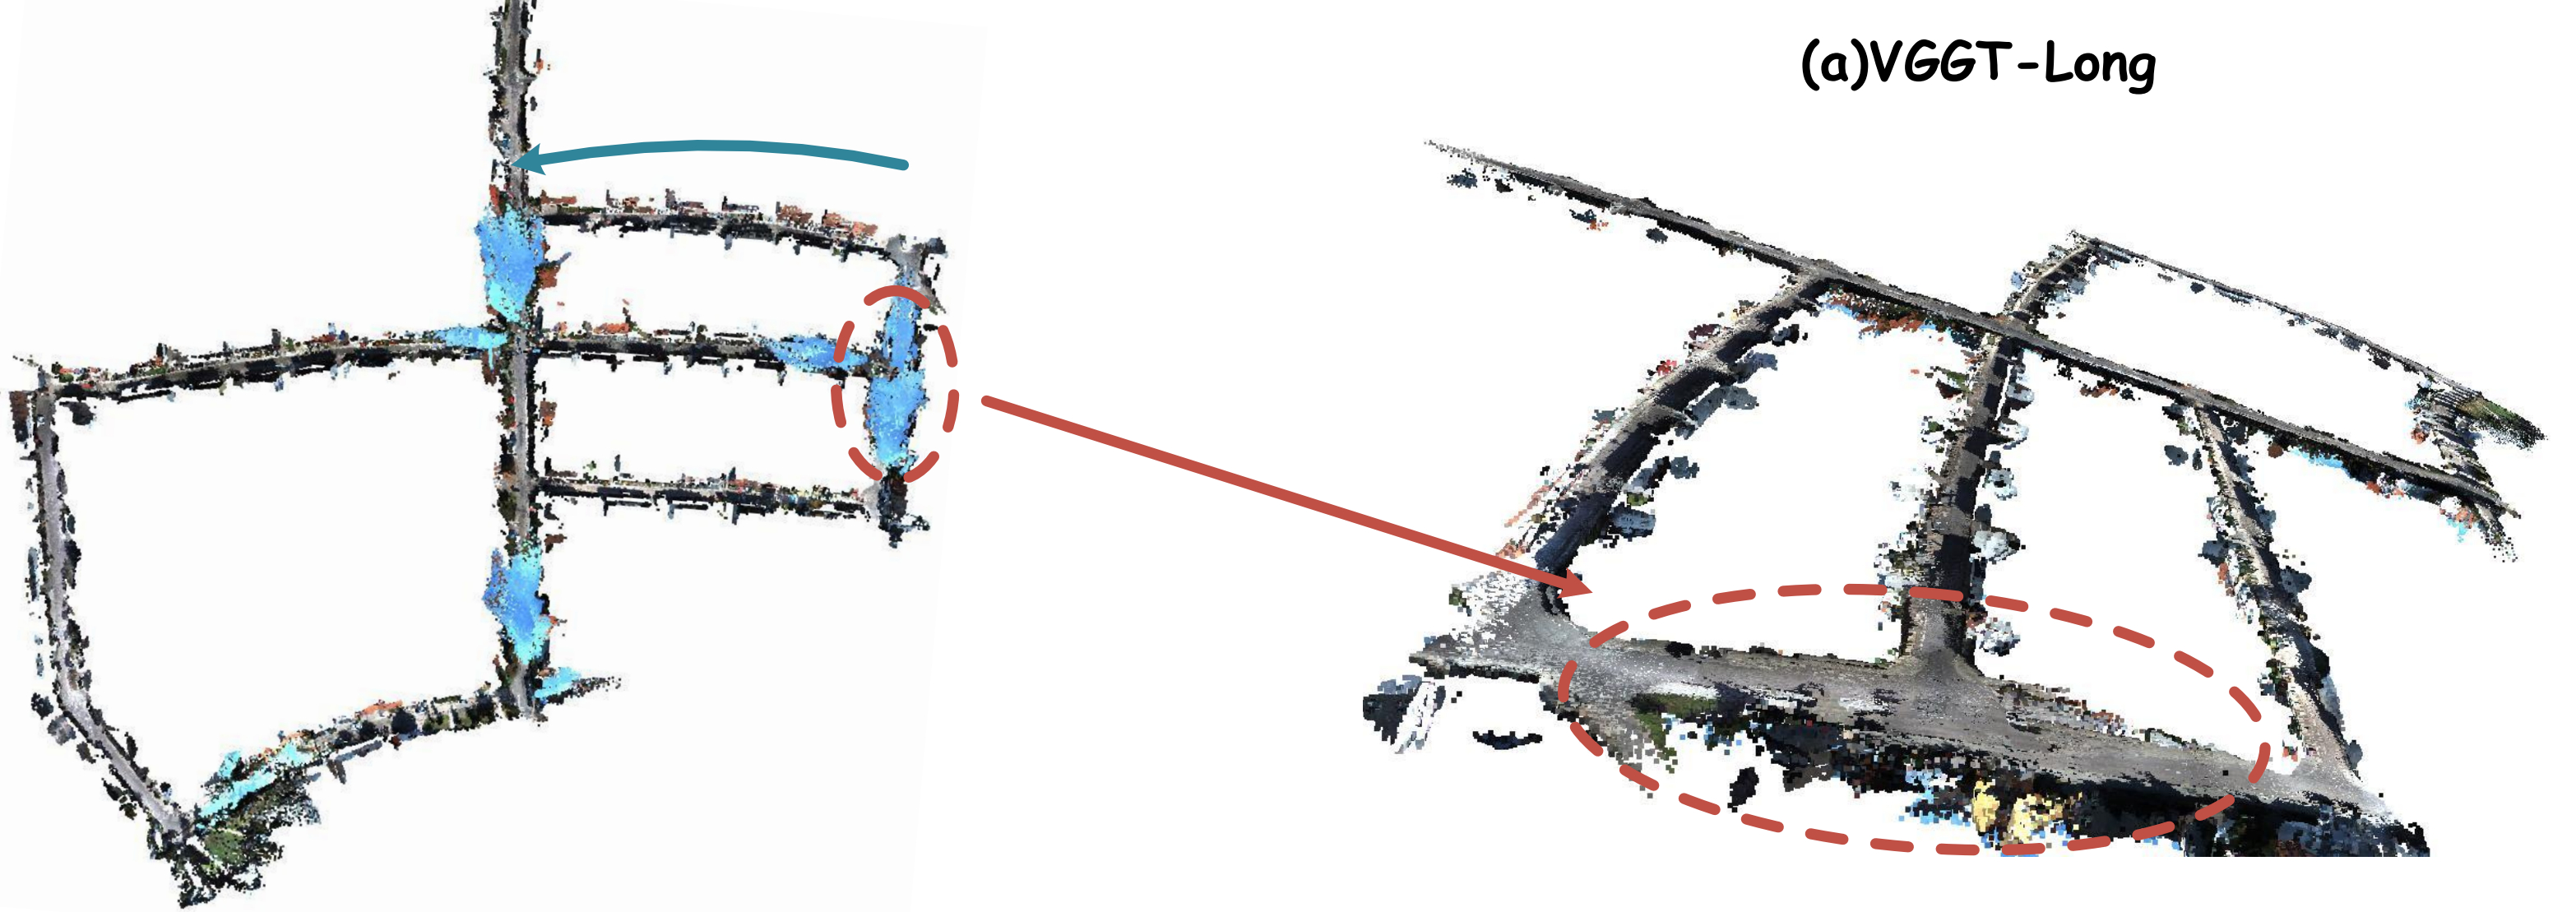

(b)VGGT-Motion

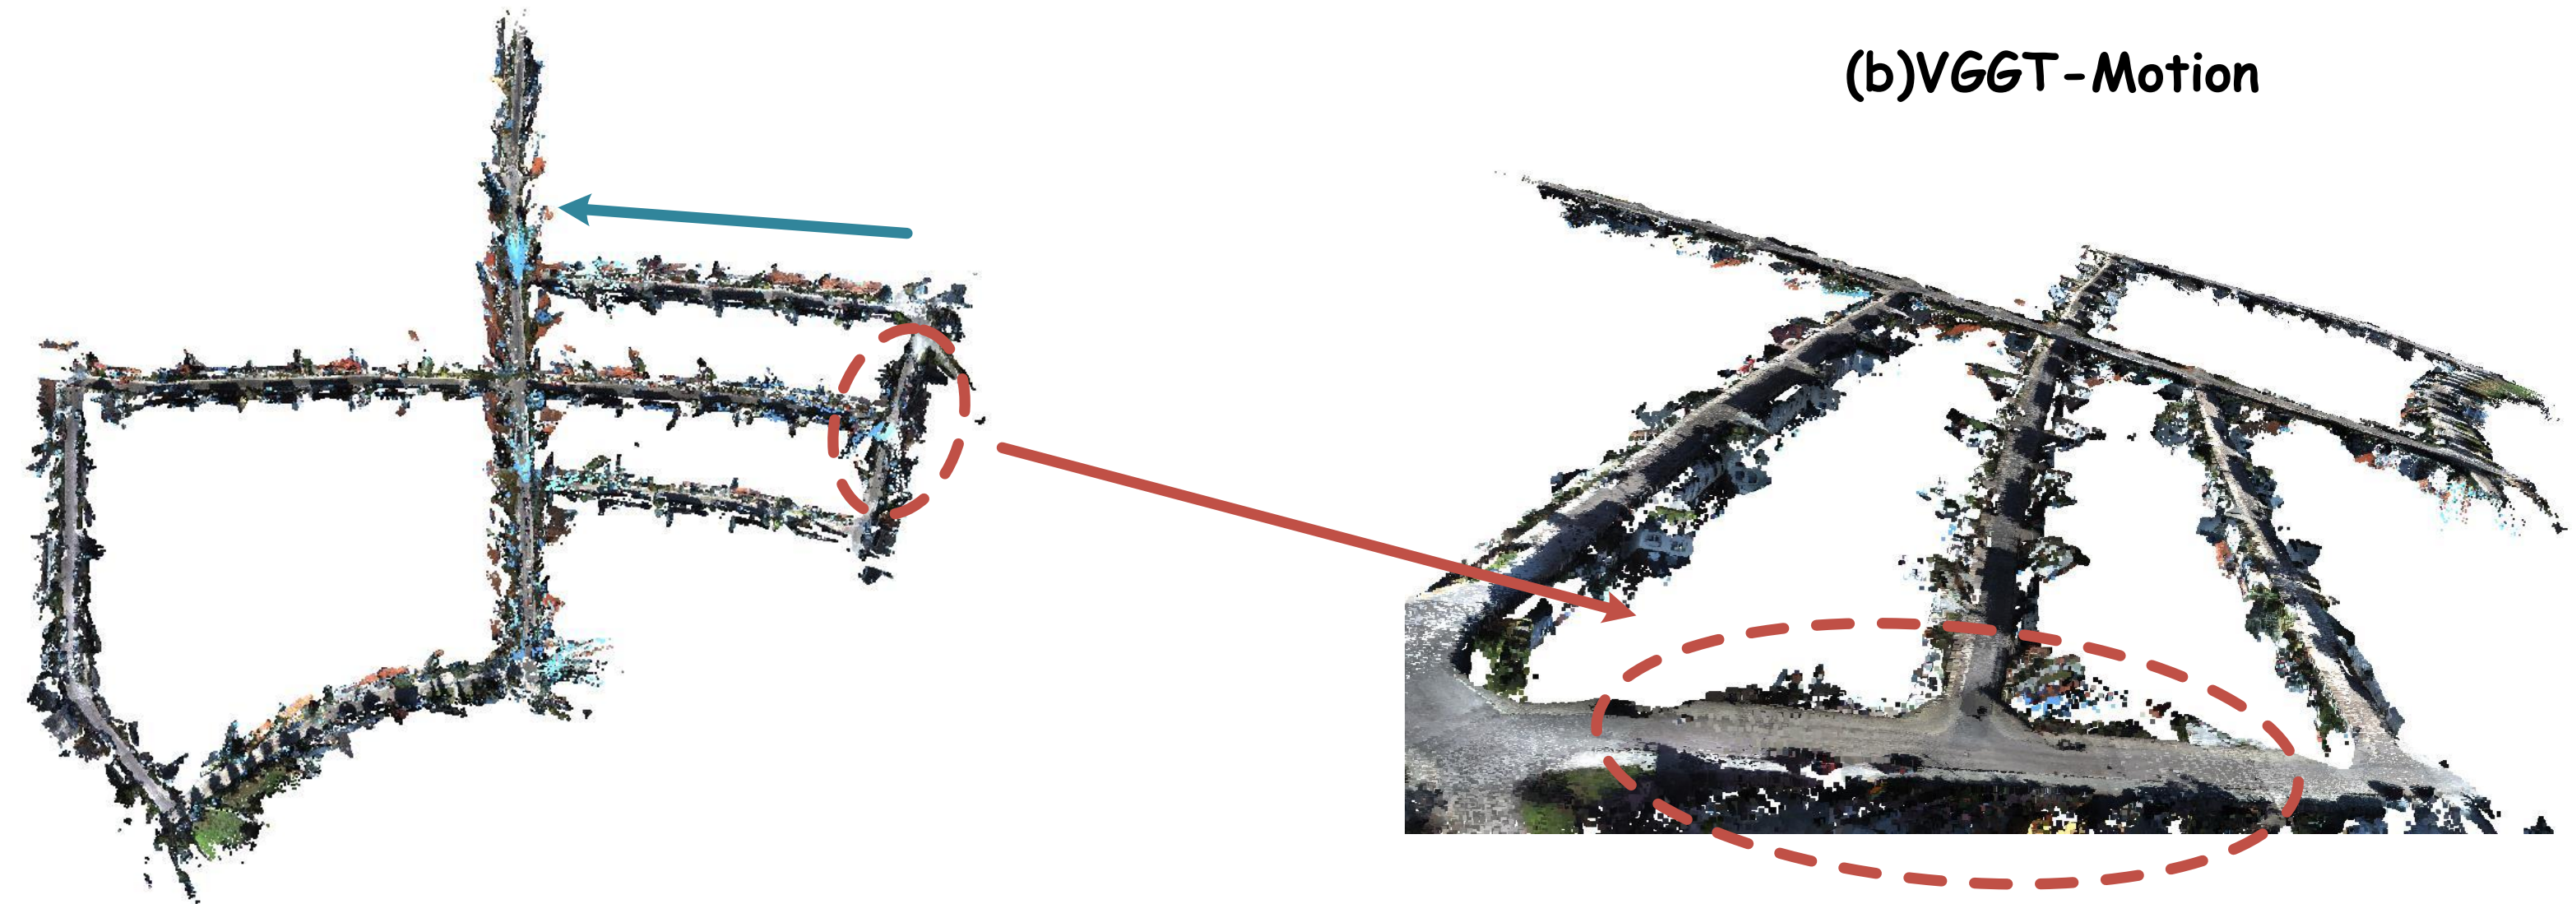



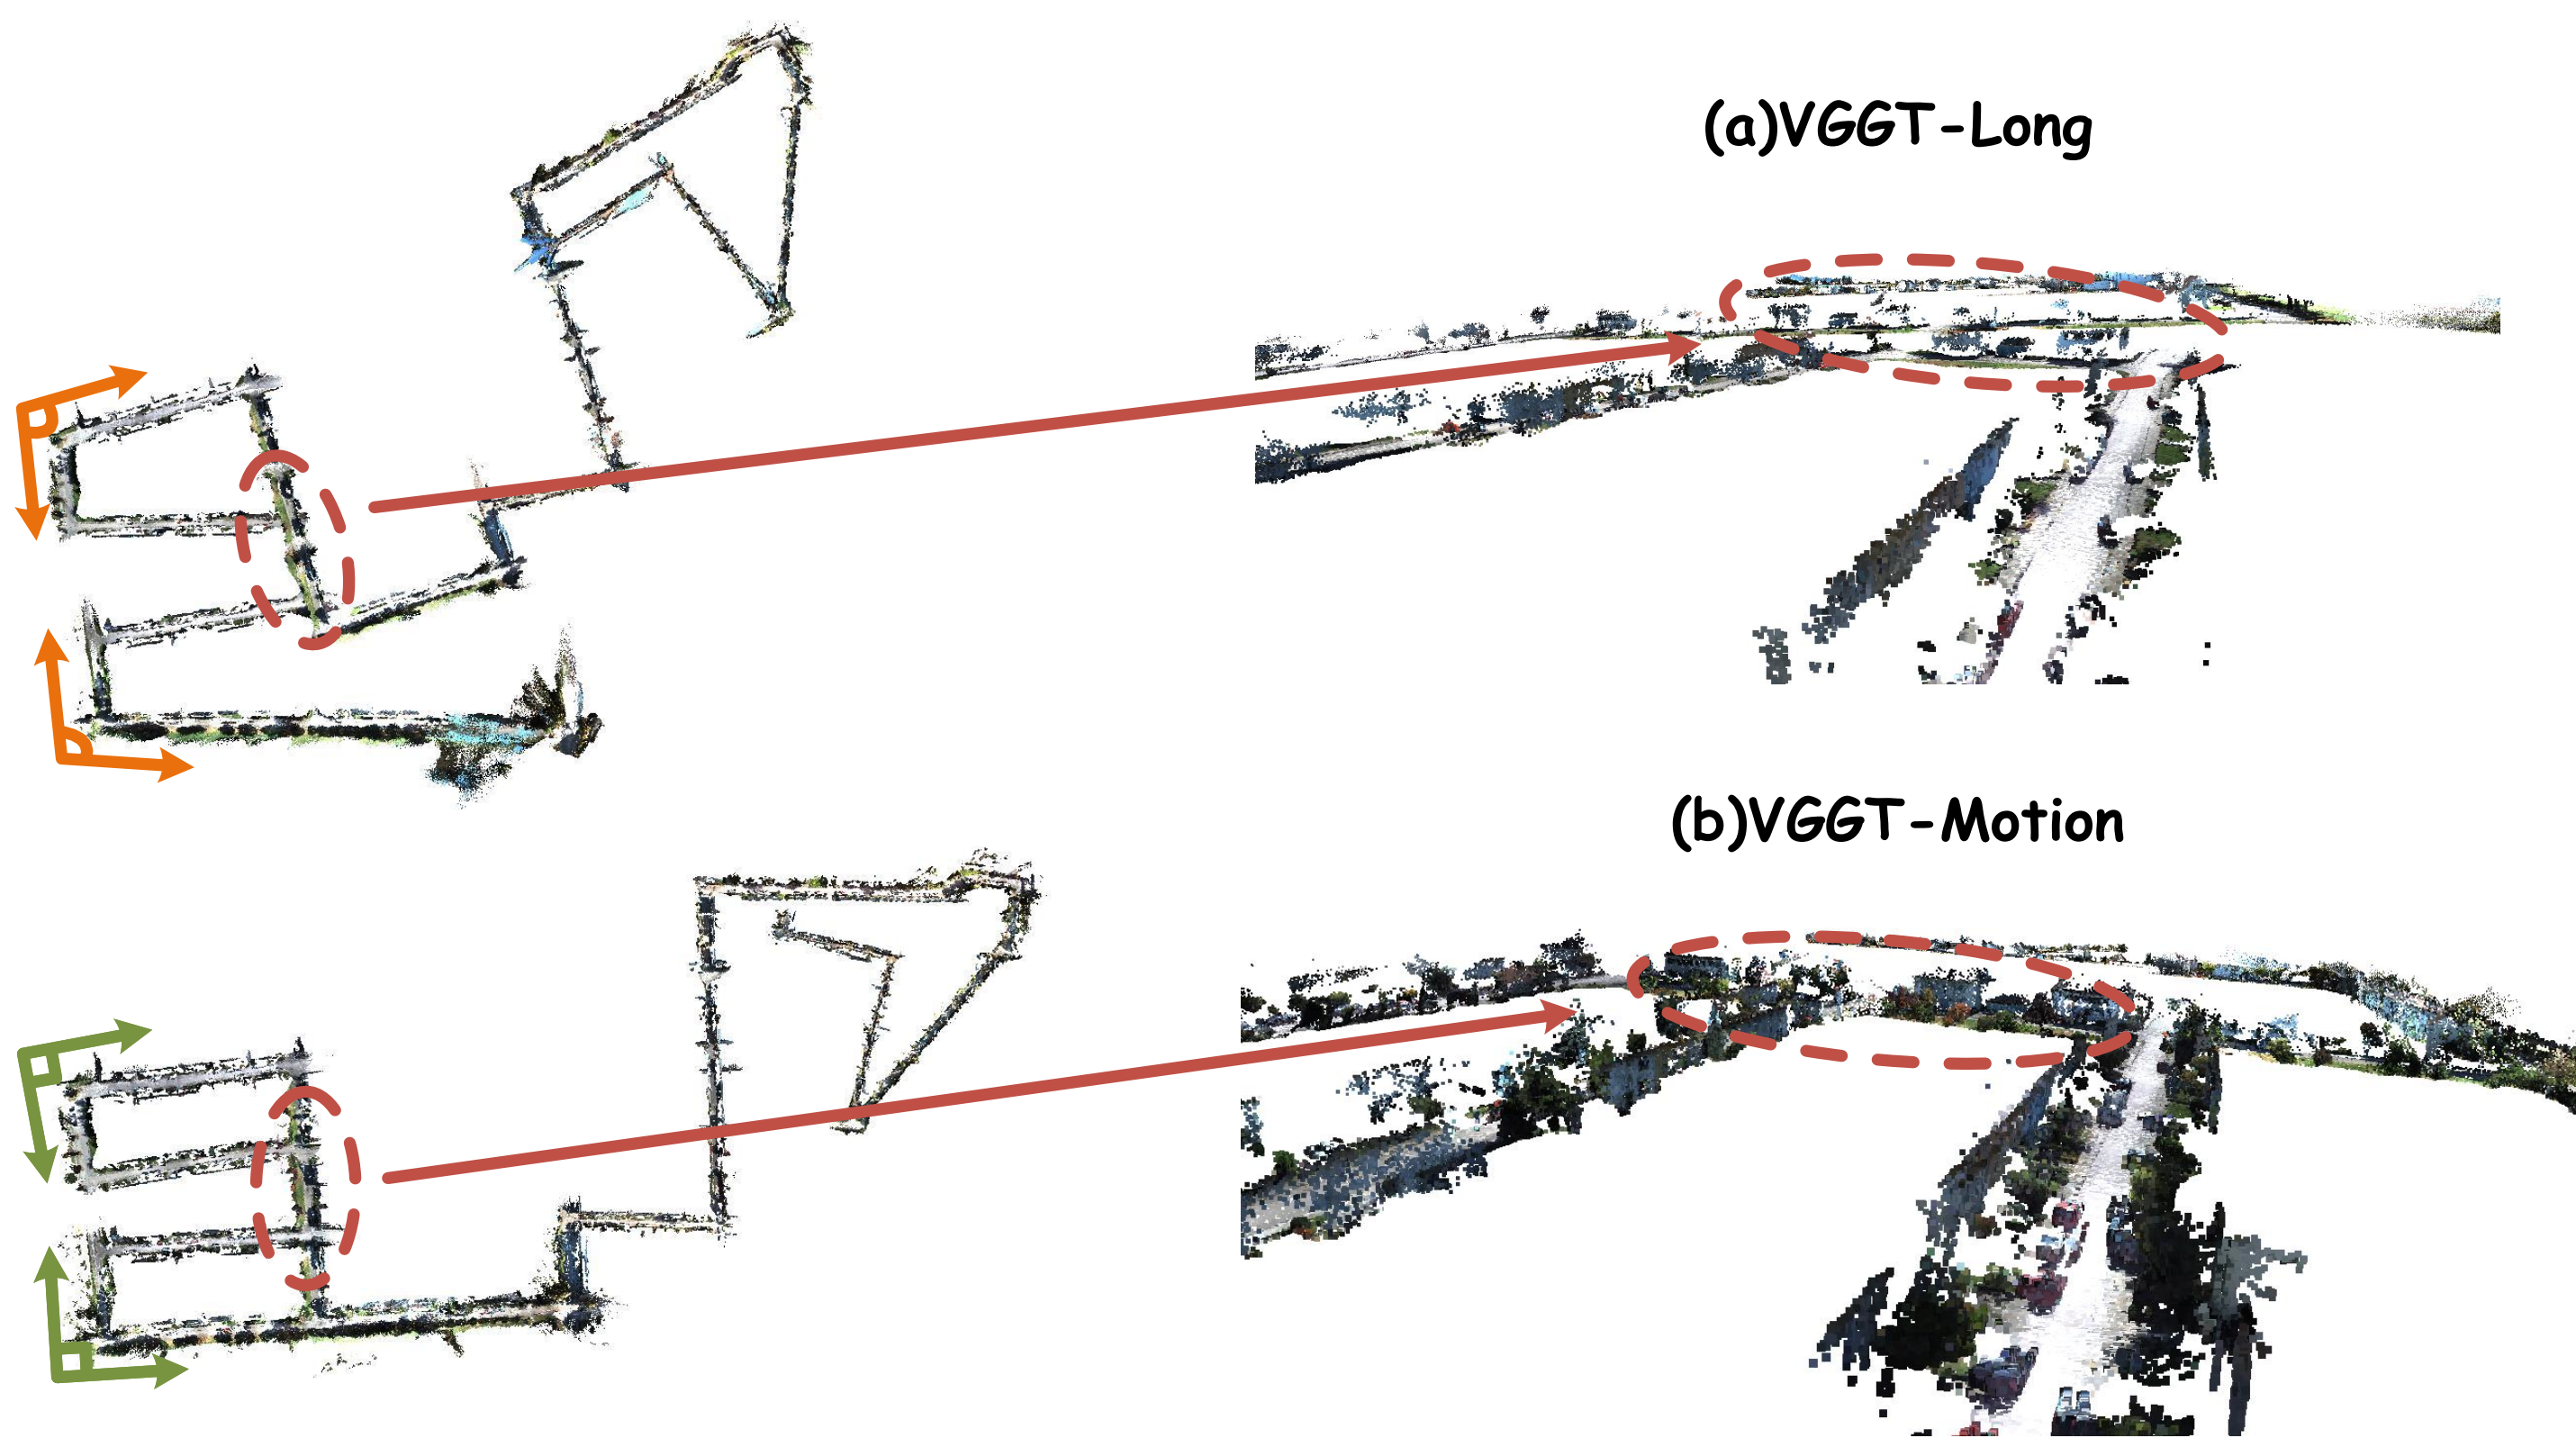

Supplement: Supplementary file 4 [file c3.pdf]
